# Supplementary material for: High resolution spectroscopy of the extended narrow-line region of IC 5063 and NGC 7212
Source: arXiv:1706.08970 ancillary file (2017-06-27)
Supplement: Supplementary file 1 [file tabelle.pdf]

## Appendix C: line fluxes and simulations

In this appendix we report the flux measurements and the results of SUMA simulations. We produced two tables for each region, the first for  $V \geq 0$  and the second for  $V < 0$ . We numbered the bins according to their velocity, starting from the bin at  $V = 0$ . For each one of them we compared the observations with the results of the models. In Sec. 1 we show the tables for IC 5063, in Sec. 2 those for NGC 7212.

## 1 IC 5063

**Table C1:** Simulation for  $v \geq 0$  of the N2 region of IC 5063. For each bin there are the observed quantities and the results of the models. The first nine rows show the comparison between the observed and the synthetic spectra, the remaining rows show the input parameters of each model.

| line                                       | bin 0 |                      | bin 1 |        | bin 2 |                      | bin 3 |                      | bin 4 |       | bin 5 |                      |
|--------------------------------------------|-------|----------------------|-------|--------|-------|----------------------|-------|----------------------|-------|-------|-------|----------------------|
|                                            | obs.  | mod.                 | obs.  | mod.   | obs.  | mod.                 | obs.  | mod.                 | obs.  | mod.  | obs.  | mod.                 |
| [O II] $\lambda$ 3727+                     | 3.04  | 3.3                  | 4.28  | 4.0    | 10.46 | 10.2                 | 38.6  | 33.3                 | 3.46  | 3.9   | 17.8  | 16.5                 |
| [Ne III] $\lambda$ 3869+                   | 1.41  | 1.34                 | 2.35  | 1.43   | 4.23  | 2.7                  | 11.73 | 4.3                  | 3.05  | 2.23  | 0.0   | 3.4                  |
| [He II] $\lambda$ 4686                     | 0.192 | 0.3                  | 0.003 | 0.2    | 0.05  | 0.14                 | 0.0   | 0.07                 | 0.0   | 0.19  | 0.0   | 0.06                 |
| [O III] $\lambda$ 5007+                    | 10.58 | 10.66                | 7.7   | 7.68   | 6.73  | 7.0                  | 10.35 | 12.5                 | 5.14  | 5.2   | 12.91 | 9.0                  |
| [O I] $\lambda$ 6300,[S II] $\lambda$ 6310 | 0.2   | 0.12                 | 0.2   | 0.1    | 0.27  | 0.11                 | 0.56  | 0.54                 | 0.53  | 0.54  | 1.54  | 0.2                  |
| H $\alpha$                                 | 2.86  | 3.2                  | 2.86  | 3.17   | 2.86  | 3.2                  | 2.86  | 4.3                  | 2.38  | 2.95  | 3.    | 4.1                  |
| [N II] $\lambda$ 6584                      | 1.51  | 1.3                  | 1.59  | 1.78   | 1.9   | 1.76                 | 2.61  | 2.46                 | 3.23  | 2.1   | 1.17  | 2.5                  |
| [S II] $\lambda$ 6716                      | 0.53  | 0.5                  | 0.45  | 0.48   | 0.52  | 0.48                 | 0.58  | 0.66                 | 0.26  | 0.25  | 15.5  | 0.86                 |
| [S II] $\lambda$ 6731                      | 0.46  | 0.6                  | 0.44  | 0.74   | 0.5   | 0.44                 | 0.78  | 0.58                 | 1.02  | 0.47  | 3.1   | 1.                   |
| FWHM(km s $^{-1}$ )                        | 0.0   | —                    | 100   | —      | 200   | —                    | 300   | —                    | 400   | —     | 500   | —                    |
| V $_s$ (km s $^{-1}$ )                     | —     | 55                   | —     | 100    | —     | 230                  | —     | 290                  | —     | 400   | —     | 530                  |
| n $_0$ (cm $^{-3}$ )                       | —     | 270                  | —     | 250    | —     | 40                   | —     | 40                   | —     | 210   | —     | 50                   |
| D(10 $^{18}$ cm)                           | —     | 0.0015               | —     | 0.0015 | —     | 0.04                 | —     | 0.06                 | —     | 0.02  | —     | 0.04                 |
| F (units $^1$ )                            | —     | 0.25                 | —     | 0.3    | —     | 0.02                 | —     | 0.002                | —     | 2.0   | —     | $1. \times 10^{-7}$  |
| O/H (10 $^{-4}$ )                          | —     | 6.6                  | —     | 6.6    | —     | 6.0                  | —     | 6.6                  | —     | 6.6   | —     | 6.0                  |
| N/H (10 $^{-4}$ )                          | —     | 1.2                  | —     | 0.8    | —     | 0.5                  | —     | 0.5                  | —     | 0.5   | —     | 1.0                  |
| Ne/H(10 $^{-4}$ )                          | —     | 1.4                  | —     | 1.6    | —     | 2.                   | —     | 2.                   | —     | 2.    | —     | 2.0                  |
| S/H (10 $^{-4}$ )                          | —     | 0.4                  | —     | 0.4    | —     | 0.1                  | —     | 0.06                 | —     | 0.06  | —     | 0.3                  |
| H $\beta$ (erg)                            | —     | $3.6 \times 10^{-4}$ | —     | 0.003  | —     | $2.3 \times 10^{-4}$ | —     | $1.1 \times 10^{-4}$ | —     | 0.056 | —     | $3.3 \times 10^{-4}$ |

$^1$  in  $10^{10}$  phot cm $^{-2}$ s $^{-1}$ eV $^{-1}$  at the Lyman limit ( $\alpha_{UV} = -1.5$ ,  $\alpha_X = -0.7$ );

**Table C2:** Simulation for  $V < 0$  of the N2 region of IC 5063. For each bin there are the observed quantities and the results of the models. The first nine rows show the comparison between the observed and the synthetic spectra, the remaining rows show the input parameters of each model.

| line                                       | bin -1 |                      | bin -2 |       | bin -3 |       | bin -4 |                      |
|--------------------------------------------|--------|----------------------|--------|-------|--------|-------|--------|----------------------|
|                                            | obs.   | mod.                 | obs.   | mod.  | obs.   | mod.  | obs.   | mod.                 |
| [O II] $\lambda$ 3727+                     | 2.92   | 2.83                 | 2.2    | 2.1   | 8.6    | 10.2  | 20.3   | 24.                  |
| [Ne III] $\lambda$ 3869+                   | 1.68   | 1.6                  | 1.13   | 1.3   | 1.53   | 3.0   | 0.74   | 1.5                  |
| [He II] $\lambda$ 4686                     | 0.14   | 0.39                 | 0.1    | 0.3   | 0.0    | 0.8   | 0.0    | 0.1                  |
| [O III] $\lambda$ 5007+                    | 11.7   | 11.9                 | 9.4    | 9.97  | 11.8   | 11.2  | 15.    | 14.                  |
| [O I] $\lambda$ 6300,[S II] $\lambda$ 6310 | 0.22   | 0.17                 | 0.21   | 0.2   | 0.11   | 1.0   | 0.2    | 0.2                  |
| H $\alpha$                                 | 2.86   | 3.18                 | 2.86   | 2.89  | 2.86   | 3.9   | 2.86   | 4.4                  |
| [N II] $\lambda$ 6584                      | 1.5    | 1.2                  | 1.77   | 1.8   | 1.53   | 3.6   | 2.13   | 2.9                  |
| [S II] $\lambda$ 6716                      | 0.63   | 0.5                  | 1.08   | 0.5   | 0.42   | 1.6   | 0.4    | 0.5                  |
| [S II] $\lambda$ 6731                      | 0.49   | 0.7                  | 0.75   | 1.2   | 0.33   | 1.2   | 0.24   | 0.6                  |
| FWHM(km s $^{-1}$ )                        | -100   | —                    | -200   | —     | -300   | —     | -400   | —                    |
| V $_s$ (km s $^{-1}$ )                     | —      | 100                  | —      | 200   | —      | 300   | —      | 400                  |
| n $_0$ (cm $^{-3}$ )                       | —      | 210                  | —      | 500   | —      | 16    | —      | 100                  |
| D(10 $^{18}$ cm)                           | —      | 0.0015               | —      | 0.004 | —      | 10.   | —      | 0.09                 |
| F (units $^1$ )                            | —      | 0.45                 | —      | 5.6   | —      | 0.6   | —      | 0.0                  |
| O/H (10 $^{-4}$ )                          | —      | 6.6                  | —      | 6.6   | —      | 5.6   | —      | 6.6                  |
| N/H (10 $^{-4}$ )                          | —      | 0.9                  | —      | 0.7   | —      | 0.5   | —      | 0.6                  |
| Ne/H(10 $^{-4}$ )                          | —      | 1.6                  | —      | 1.2   | —      | 1.0   | —      | 0.6                  |
| S/H (10 $^{-4}$ )                          | —      | 0.6                  | —      | 0.6   | —      | 0.1   | —      | 0.05                 |
| H $\beta$ (erg)                            | —      | $7.4 \times 10^{-4}$ | —      | 0.09  | —      | 0.004 | —      | $3.8 \times 10^{-4}$ |

$^1$  in  $10^{10}$  phot cm $^{-2}$ s $^{-1}$ eV $^{-1}$  at the Lyman limit ( $\alpha_{UV} = -1.5$ ,  $\alpha_X = -0.7$ );

**Table C3:** Simulation for  $v \geq 0$  of the N1 region of IC 5063. For each bin there are the observed quantities and the results of the models. The first nine rows show the comparison between the observed and the synthetic spectra, the remaining rows show the input parameters of each model.

|                                            | bin 0 |                     | bin 1 |                      | bin 2 |       | bin 3 |      | bin 4 |       | bin 5 |       | bin 6 |       |
|--------------------------------------------|-------|---------------------|-------|----------------------|-------|-------|-------|------|-------|-------|-------|-------|-------|-------|
| line                                       | obs.  | mod.                | obs.  | mod.                 | obs.  | mod.  | obs.  | mod. | obs.  | mod.  | obs.  | mod.  | obs.  | mod.  |
| [O II] $\lambda$ 3727+                     | 2.6   | 2.4                 | 3.20  | 3.25                 | 4.14  | 4.4   | 4.3   | 4.1  | 4.54  | 4.7   | 3.16  | 3.1   | 1.83  | 1.9   |
| [Ne III] $\lambda$ 3869+                   | 1.26  | 1.1                 | 2.1   | 1.1                  | 1.9   | 2.4   | 1.17  | 1.3  | 1.56  | 1.2   | 0.95  | 1.0   | 0.5   | 0.76  |
| [He II] $\lambda$ 4686                     | 0.165 | 0.4                 | 0.1   | 0.24                 | 0.04  | 0.26  | 0.0   | 0.2  | 0.    | 0.2   | 0.0   | 0.17  | 0.0   | 0.14  |
| [O III] $\lambda$ 5007+                    | 10.26 | 10.2                | 7.91  | 7.5                  | 7.11  | 7.1   | 5.6   | 5.3  | 5.48  | 5.53  | 5.9   | 5.9   | 5.0   | 5.1   |
| [O I] $\lambda$ 6300,[S II] $\lambda$ 6310 | 0.31  | 0.15                | 0.38  | 0.15                 | 0.44  | 0.9   | 0.46  | 0.5  | 0.43  | 0.45  | 0.45  | 0.5   | 0.66  | 0.7   |
| H $\alpha$                                 | 2.86  | 3.0                 | 2.86  | 3.2                  | 2.86  | 2.96  | 2.86  | 3.   | 2.86  | 3.0   | 2.86  | 3.    | 2.56  | 3.    |
| [N II] $\lambda$ 6584                      | 1.65  | 1.7                 | 1.81  | 1.94                 | 1.8   | 1.6   | 1.78  | 1.5  | 1.9   | 2.0   | 2.47  | 2.6   | 3.44  | 2.4   |
| [S II] $\lambda$ 6716                      | 0.66  | 0.7                 | 0.74  | 0.6                  | 0.7   | 1.0   | 0.6   | 0.55 | 0.72  | 0.55  | 0.46  | 0.42  | 1.33  | 0.6   |
| [S II] $\lambda$ 6731                      | 0.61  | 0.8                 | 0.71  | 0.84                 | 0.72  | 1.4   | 0.64  | 0.88 | 0.66  | 0.84  | 0.86  | 0.7   | 1.05  | 1.0   |
| FWHM(km s $^{-1}$ )                        | 0.0   | —                   | 100   | —                    | 200   | —     | 300   | —    | 400   | —     | 500   | —     | 600   | —     |
| V $_s$ (km s $^{-1}$ )                     | —     | 50                  | —     | 100                  | —     | 220   | —     | 300  | —     | 400   | —     | 500   | —     | 600   |
| n $_0$ (cm $^{-3}$ )                       | —     | 240                 | —     | 210                  | —     | 300   | —     | 300  | —     | 150   | —     | 140   | —     | 130   |
| D(10 $^{18}$ cm)                           | —     | 0.0015              | —     | 0.0016               | —     | 0.6   | —     | 0.6  | —     | 1.    | —     | 0.1   | —     | 0.2   |
| F (units $^1$ )                            | —     | 0.22                | —     | 0.26                 | —     | 2.4   | —     | 2.4  | —     | 1.4   | —     | 2.5   | —     | 4     |
| O/H (10 $^{-4}$ )                          | —     | 6.6                 | —     | 6.7                  | —     | 6.3   | —     | 6.6  | —     | 6.6   | —     | 6.6   | —     | 6.6   |
| N/H (10 $^{-4}$ )                          | —     | 1.2                 | —     | 1.2                  | —     | 0.5   | —     | 0.5  | —     | 0.5   | —     | 0.9   | —     | 1.2   |
| Ne/H(10 $^{-4}$ )                          | —     | 1.4                 | —     | 1.4                  | —     | 1.4   | —     | 1.   | —     | 1.    | —     | 1.    | —     | 1.    |
| S/H (10 $^{-4}$ )                          | —     | 0.6                 | —     | 0.6                  | —     | 0.07  | —     | 0.07 | —     | 0.07  | —     | 0.1   | —     | 0.2   |
| H $\beta$ (erg)                            | —     | $1. \times 10^{-4}$ | —     | $9.2 \times 10^{-4}$ | —     | 0.054 | —     | 0.06 | —     | 0.038 | —     | 0.082 | —     | 0.155 |

$^1$  in  $10^{10}$  phot cm $^{-2}$ s $^{-1}$ eV $^{-1}$  at the Lyman limit ( $\alpha_{UV} = -1.5$ ,  $\alpha_X = -0.7$ );

**Table C4:** Simulation for  $V < 0$  of the N1 region of IC 5063. For each bin there are the observed quantities and the results of the models. The first nine rows show the comparison between the observed and the synthetic spectra, the remaining rows show the input parameters of each model.

| line                                       | bin -1 |                      | bin -2 |                      | bin -3 |       | bin -4 |       | bin -5 |       | bin -6 |       | bin -7 |        |
|--------------------------------------------|--------|----------------------|--------|----------------------|--------|-------|--------|-------|--------|-------|--------|-------|--------|--------|
|                                            | obs.   | mod.                 | obs.   | mns1-2               | obs.   | mod.  | obs.   | mod.  | obs.   | mod.  | obs.   | mod.  | obs.   | mod.   |
| [O II] $\lambda$ 3727+                     | 2.5    | 2.56                 | 2.18   | 2.3                  | 2.44   | 2.4   | 2.61   | 2.9   | 2.82   | 2.81  | 2.62   | 2.9   | 0.65   | 0.82   |
| [Ne III] $\lambda$ 3869+                   | 1.17   | 1.18                 | 1.1    | 1.3                  | 1.11   | 1.4   | 1.13   | 1.4   | 1.32   | 1.33  | 1.3    | 1.4   | 1.14   | 0.94   |
| [He II] $\lambda$ 4686                     | 0.127  | 0.4                  | 0.127  | 0.38                 | 0.137  | 0.35  | 0.129  | 0.27  | 0.03   | 0.29  | 0.0    | 0.3   | 0.0    | 0.5    |
| [O III] $\lambda$ 5007+                    | 10.84  | 10.7                 | 10.6   | 10.5                 | 10.76  | 10.9  | 10.2   | 10.7  | 9.65   | 9.8   | 11.0   | 10.9  | 10.6   | 10.5   |
| [O I] $\lambda$ 6300,[S II] $\lambda$ 6310 | 0.26   | 0.15                 | 0.26   | 0.15                 | 0.26   | 0.2   | 0.34   | 0.22  | 0.48   | 0.42  | 0.55   | 0.2   | 0.35   | 0.05   |
| H $\alpha$                                 | 2.86   | 3.1                  | 2.86   | 2.97                 | 2.86   | 2.89  | 2.86   | 2.88  | 2.86   | 2.9   | 2.86   | 2.88  | 2.86   | 2.9    |
| [N II] $\lambda$ 6584                      | 1.7    | 1.6                  | 1.72   | 1.5                  | 1.63   | 1.8   | 1.79   | 2.0   | 1.86   | 2.0   | 1.78   | 2.0   | 0.98   | 0.86   |
| [S II] $\lambda$ 6716                      | 0.85   | 0.74                 | 0.92   | 0.4                  | 0.74   | 0.7   | 0.68   | 0.7   | 0.69   | 0.61  | 0.8    | 0.6   | 0.75   | 0.3    |
| [S II] $\lambda$ 6731                      | 0.75   | 0.63                 | 0.75   | 0.7                  | 0.66   | 1.3   | 0.67   | 1.5   | 0.85   | 1.28  | 0.78   | 1.15  | 0.59   | 0.65   |
| FWHM(km s $^{-1}$ )                        | -100   | —                    | -200   | —                    | -300   | —     | -400   | —     | -500   | —     | -600   | —     | -700   | —      |
| V $_s$ (km s $^{-1}$ )                     | —      | 80                   | —      | 200                  | —      | 300   | —      | 400   | —      | 500   | —      | 600   | —      | 700    |
| n $_0$ (cm $^{-3}$ )                       | —      | 260                  | —      | 250                  | —      | 240   | —      | 260   | —      | 280   | —      | 260   | —      | 340    |
| D(10 $^{18}$ cm)                           | —      | 0.0015               | —      | 0.0025               | —      | 0.011 | —      | 0.011 | —      | 0.011 | —      | 0.011 | —      | 0.0065 |
| F (units $^1$ )                            | —      | 0.5                  | —      | 1.1                  | —      | 3.7   | —      | 5.    | —      | 7.8   | —      | 8.3   | —      | 6.     |
| O/H (10 $^{-4}$ )                          | —      | 6.6                  | —      | 6.6                  | —      | 6.6   | —      | 6.6   | —      | 6.6   | —      | 6.6   | —      | 6.6    |
| N/H (10 $^{-4}$ )                          | —      | 1.2                  | —      | 1.2                  | —      | 1.2   | —      | 0.8   | —      | 0.8   | —      | 0.6   | —      | 0.6    |
| Ne/H(10 $^{-4}$ )                          | —      | 1.4                  | —      | 1.4                  | —      | 1.4   | —      | 1.    | —      | 1.    | —      | 1.    | —      | 1.     |
| S/H (10 $^{-4}$ )                          | —      | 0.6                  | —      | 0.6                  | —      | 0.6   | —      | 0.3   | —      | 0.3   | —      | 0.3   | —      | 0.3    |
| H $\beta$ (erg)                            | —      | $8.7 \times 10^{-4}$ | —      | $3.4 \times 10^{-3}$ | —      | 0.057 | —      | 0.1   | —      | 0.18  | —      | 0.21  | —      | 0.3    |

<sup>1</sup> in 10 $^{10}$  phot cm $^{-2}$ s $^{-1}$ eV $^{-1}$  at the Lyman limit ( $\alpha_{UV} = -1.5$ ,  $\alpha_X = -0.7$ );

**Table C5:** Simulation for  $v \geq 0$  of the N0 region of IC 5063. For each bin there are the observed quantities and the results of the models. The first nine rows show the comparison between the observed and the synthetic spectra, the remaining rows show the input parameters of each model.

|                                            | bin 0 |       | bin 1 |      | bin 2 |      | bin 3 |      | bin 4 |       | bin 5 |       | bin 6 |       | bin 7 |      | bin 8 |      |
|--------------------------------------------|-------|-------|-------|------|-------|------|-------|------|-------|-------|-------|-------|-------|-------|-------|------|-------|------|
| line                                       | obs.  | mod.  | obs.  | mod. | obs.  | mod. | obs.  | mod. | obs.  | mod.  | obs.  | mod.  | obs.  | mod.  | obs.  | mod. | obs.  | mod. |
| [O II] $\lambda$ 3727+                     | 3.5   | 3.8   | 3.25  | 3.0  | 3.67  | 3.3  | 3.89  | 4.0  | 5.2   | 5.36  | 6.26  | 6.3   | 3.35  | 3.7   | 3.64  | 3.3  | 3.97  | 3.96 |
| [Ne III] $\lambda$ 3869+                   | 1.64  | 1.3   | 1.58  | 1.56 | 1.3   | 1.58 | 1.34  | 1.7  | 1.81  | 1.72  | 1.47  | 1.6   | 1.25  | 1.2   | 1.23  | 1.29 | 0.9   | 1.2  |
| [He II] $\lambda$ 4686                     | 0.138 | 0.29  | 0.11  | 0.26 | 0.07  | 0.2  | 0.08  | 0.2  | 0.1   | 0.25  | 0.15  | 0.3   | 0.08  | 0.17  | 0.11  | 0.2  | 0.0   | 0.2  |
| [O III] $\lambda$ 5007+                    | 9.5   | 9.4   | 8.87  | 8.9  | 6.48  | 6.9  | 6.95  | 6.84 | 7.22  | 7.1   | 10.7  | 10.7  | 5.4   | 5.48  | 6.3   | 6.6  | 7.6   | 7.89 |
| [O I] $\lambda$ 6300,[S II] $\lambda$ 6310 | 0.41  | 0.32  | 0.5   | 0.7  | 0.57  | 0.7  | 0.55  | 0.7  | 0.55  | 0.8   | 0.56  | 0.6   | 0.5   | 0.3   | 0.47  | 0.4  | 0.64  | 0.5  |
| H $\alpha$                                 | 2.86  | 2.9   | 2.86  | 3.0  | 2.86  | 2.86 | 2.86  | 2.98 | 2.86  | 3.0   | 2.86  | 2.99  | 2.86  | 3.18  | 2.86  | 3.18 | 2.86  | 3.2  |
| [N II] $\lambda$ 6584                      | 1.85  | 1.6   | 2.1   | 1.7  | 2.27  | 2.1  | 2.18  | 2.3  | 2.0   | 2.2   | 1.9   | 2.1   | 1.93  | 2.    | 2.2   | 2.   | 2.9   | 2.8  |
| [S II] $\lambda$ 6716                      | 0.87  | 0.7   | 1.1   | 1.17 | 1.34  | 0.8  | 1.46  | 0.24 | 1.33  | 1.43  | 1.1   | 1.0   | 0.98  | 0.6   | 0.63  | 0.86 | 0.83  | 1.   |
| [S II] $\lambda$ 6731                      | 0.72  | 1.0   | 0.86  | 1.76 | 1.0   | 1.34 | 0.97  | 1.82 | 0.88  | 1.9   | 0.4   | 1.2   | 0.91  | 0.9   | 0.95  | 1.2  | 1.19  | 1.3  |
| FWHM(km s <sup>-1</sup> )                  | 0.0   | —     | 100   | —    | 200   | —    | 300   | —    | 400   | —     | 500   | —     | 600   | —     | 700   | —    | 800   | —    |
| V <sub>s</sub> (km s <sup>-1</sup> )       | —     | 58    | —     | 100  | —     | 210  | —     | 280  | —     | 380   | —     | 490   | —     | 600   | —     | 700  | —     | 800  |
| n <sub>0</sub> (cm <sup>-3</sup> )         | —     | 420   | —     | 580  | —     | 440  | —     | 300  | —     | 120   | —     | 60    | —     | 80    | —     | 67   | —     | 50   |
| D(10 <sup>18</sup> cm)                     | —     | 0.1   | —     | 0.95 | —     | 0.95 | —     | 1.0  | —     | 2.0   | —     | 2.0   | —     | 2.5   | —     | 2.5  | —     | 2.5  |
| F (units <sup>1</sup> )                    | —     | 2.1   | —     | 5.   | —     | 4.   | —     | 3.   | —     | 1.2   | —     | 0.9   | —     | 1.3   | —     | 2.   | —     | 2.3  |
| O/H (10 <sup>-4</sup> )                    | —     | 6.6   | —     | 6.6  | —     | 6.6  | —     | 6.6  | —     | 6.6   | —     | 6.6   | —     | 6.6   | —     | 6.6  | —     | 6.6  |
| N/H (10 <sup>-4</sup> )                    | —     | 0.5   | —     | 0.5  | —     | 0.5  | —     | 0.5  | —     | 0.5   | —     | 0.5   | —     | 0.7   | —     | 0.8  | —     | 0.9  |
| Ne/H(10 <sup>-4</sup> )                    | —     | 1.2   | —     | 1.2  | —     | 1.2  | —     | 1.2  | —     | 1.2   | —     | 1.0   | —     | 1.3   | —     | 1.3  | —     | 1    |
| S/H (10 <sup>-4</sup> )                    | —     | 0.12  | —     | 0.12 | —     | 0.12 | —     | 0.12 | —     | 0.12  | —     | 0.08  | —     | 0.1   | —     | 0.16 | —     | 0.16 |
| H $\beta$ (erg)                            | —     | 0.068 | —     | 0.12 | —     | 0.09 | —     | 0.07 | —     | 0.028 | —     | 0.017 | —     | 0.041 | —     | 0.07 | —     | 0.5  |

<sup>1</sup> in 10<sup>10</sup> phot cm<sup>-2</sup>s<sup>-1</sup>eV<sup>-1</sup> at the Lyman limit ( $\alpha_{UV} = -1.5$ ,  $\alpha_X = -0.7$ );

**Table C6:** Simulation for  $V < 0$  of the N0 region of IC 5063. For each bin there are the observed quantities and the results of the models. The first nine rows show the comparison between the observed and the synthetic spectra, the remaining rows show the input parameters of each model.

|                                            | bin -1 |         | bin -2 |       | bin -3 |       | bin -4 |       | bin -5 |      | bin -6 |      | bin -7 |      | bin -8 |      |
|--------------------------------------------|--------|---------|--------|-------|--------|-------|--------|-------|--------|------|--------|------|--------|------|--------|------|
| line                                       | obs.   | mns01   | obs.   | mod.  | obs.   | mod.  | obs.   | mod.  | obs.   | mod. | obs.   | mod. | obs.   | mod. | obs.   | mod. |
| [O II] $\lambda$ 3727+                     | 2.83   | 2.84    | 2.52   | 2.5   | 2.27   | 2.25  | 2.44   | 2.6   | 2.25   | 2.3  | 1.81   | 1.76 | 2.55   | 2.4  | 4.18   | 4.   |
| [Ne III] $\lambda$ 3869+                   | 1.54   | 1.3     | 1.4    | 1.2   | 1.2    | 1.28  | 1.14   | 1.3   | 1.03   | 1.47 | 1.11   | 1.15 | 1.0    | 1.37 | 1.6    | 1.4  |
| [He II] $\lambda$ 4686                     | 0.09   | 0.3     | 0.11   | 0.36  | 0.11   | 0.36  | 0.09   | 0.3   | 0.12   | 0.26 | 0.1    | 0.3  | 0.0    | 0.5  | 0.0    | 0.6  |
| [O III] $\lambda$ 5007+                    | 10.43  | 10.5    | 9.64   | 9.85  | 10.33  | 10.54 | 10.2   | 10.5  | 9.66   | 9.84 | 9.97   | 10.  | 10.72  | 10.8 | 9.64   | 9.5  |
| [O I] $\lambda$ 6300,[S II] $\lambda$ 6310 | 0.33   | 0.15    | 0.35   | 0.14  | 0.35   | 0.16  | 0.38   | 0.17  | 0.43   | 0.5  | 0.5    | 0.45 | 0.45   | 0.5  | 0.3    | 0.5  |
| H $\alpha$                                 | 2.86   | 3.2     | 2.86   | 2.9   | 2.86   | 2.9   | 2.86   | 2.9   | 2.86   | 3.   | 2.86   | 3.   | 2.86   | 3.2  | 2.86   | 3.3  |
| [N II] $\lambda$ 6584                      | 1.75   | 1.74    | 1.8    | 1.9   | 1.72   | 2.    | 1.8    | 1.95  | 2.07   | 2.3  | 2.49   | 2.74 | 2.5    | 2.5  | 2.5    | 2.7  |
| [S II] $\lambda$ 6716                      | 0.83   | 0.46    | 0.89   | 0.67  | 0.77   | 0.57  | 0.73   | 0.73  | 0.85   | 0.3  | 0.95   | 0.5  | 0.88   | 0.4  | 0.64   | 0.4  |
| [S II] $\lambda$ 6731                      | 0.68   | 0.680.7 | 1.16   | 0.6   | 1.1    | 0.6   | 0.48   | 0.69  | 0.6    | 0.53 | 0.97   | 0.73 | 0.8    | 0.47 | 0.77   |      |
| FWHM(km s <sup>-1</sup> )                  | -100   | —       | -200   | —     | -300   | —     | -400   | —     | -500   | —    | -600   | —    | -700   | —    | -800   | —    |
| V <sub>s</sub> (km s <sup>-1</sup> )       | —      | 100     | —      | 200   | —      | 300   | —      | 400   | —      | 500  | —      | 600  | —      | 700  | —      | 800  |
| n <sub>0</sub> (cm <sup>-3</sup> )         | —      | 230     | —      | 200   | —      | 200   | —      | 200   | —      | 260  | —      | 247  | —      | 240  | —      | 170  |
| D(10 <sup>18</sup> cm)                     | —      | 0.0015  | —      | 0.012 | —      | 0.012 | —      | 0.012 | —      | 0.05 | —      | 0.05 | —      | 0.06 | —      | 0.11 |
| F (units <sup>1</sup> )                    | —      | 0.45    | —      | 1.5   | —      | 2.5   | —      | 3.    | —      | 12.2 | —      | 19.  | —      | 53.  | —      | 53.  |
| O/H (10 <sup>-4</sup> )                    | —      | 6.6     | —      | 6.6   | —      | 6.6   | —      | 6.6   | —      | 6.4  | —      | 6.4  | —      | 6.4  | —      | 6.4  |
| N/H (10 <sup>-4</sup> )                    | —      | 1.2     | —      | 1.0   | —      | 1.0   | —      | 0.8   | —      | 0.7  | —      | 0.9  | —      | 0.7  | —      | 0.6  |
| Ne/H(10 <sup>-4</sup> )                    | —      | 1.4     | —      | 1.4   | —      | 1.4   | —      | 1.3   | —      | 1.0  | —      | 0.8  | —      | 0.8  | —      | 0.8  |
| S/H (10 <sup>-4</sup> )                    | —      | 0.6     | —      | 0.62  | —      | 0.6   | —      | 0.6   | —      | 0.1  | —      | 0.2  | —      | 0.2  | —      | 0.2  |
| H $\beta$ (erg)                            | —      | 0.001   | —      | 0.02  | —      | 0.035 | —      | 0.05  | —      | 0.29 | —      | 0.43 | —      | 0.87 | —      | 0.78 |

<sup>1</sup> in 10<sup>10</sup> phot cm<sup>-2</sup>s<sup>-1</sup>eV<sup>-1</sup> at the Lyman limit ( $\alpha_{UV} = -1.5$ ,  $\alpha_X = -0.7$ );



**Table C7:** Simulation for  $v \geq 0$  of the CN region of IC 5063. For each bin there are the observed quantities and the results of the models. The first nine rows show the comparison between the observed and the synthetic spectra, the remaining rows show the input parameters of each model.

|                                            | bin 0 |        | bin 1 |        | bin 2 |      | bin 3 |        | bin 4 |      | bin 5 |       | bin 6 |       | bin 7 |       |
|--------------------------------------------|-------|--------|-------|--------|-------|------|-------|--------|-------|------|-------|-------|-------|-------|-------|-------|
| line                                       | obs.  | mod.   | obs.  | mod.   | obs.  | mod. | obs.  | mod.   | obs.  | mod. | obs.  | mod.  | obs.  | mod.  | obs.  | mod.  |
| [O II] $\lambda$ 3727+                     | 3.3   | 3.0    | 3.    | 3.3    | 4.4   | 4.6  | 4.65  | 4.5    | 6.0   | 5.7  | 7.75  | 7.0   | 6.87  | 6.5   | 4.25  | 4.1   |
| [Ne III] $\lambda$ 3869+                   | 1.4   | 1.14   | 1.4   | 1.47   | 1.3   | 1.7  | 1.6   | 1.6    | 1.93  | 2.0  | 2.2   | 1.5   | 2.58  | 2.    | 1.49  | 1.45  |
| [He II] $\lambda$ 4686                     | 0.22  | 0.4    | 0.2   | 0.3    | 0.13  | 0.29 | 0.08  | 0.24   | 0.07  | 0.29 | 0.03  | 0.29  | 0.0   | 0.26  | 0.0   | 0.2   |
| [O III] $\lambda$ 5007+                    | 13.0  | 13.3   | 14.4  | 14.6   | 9.2   | 9.46 | 7.36  | 7.2    | 8.3   | 8.6  | 9.2   | 9.38  | 7.56  | 7.8   | 7.52  | 7.5   |
| [O I] $\lambda$ 6300,[S II] $\lambda$ 6310 | 0.36  | 0.2    | 0.34  | 0.36   | 0.44  | 0.8  | 0.53  | 0.6    | 0.49  | 0.7  | 0.56  | 0.6   | 0.51  | 0.6   | 0.49  | 0.65  |
| H $\alpha$                                 | 2.87  | 3.0    | 2.86  | 3.4    | 2.86  | 2.9  | 2.86  | 2.94   | 2.86  | 2.86 | 2.86  | 2.95  | 2.86  | 2.95  | 2.86  | 2.95  |
| [N II] $\lambda$ 6584                      | 1.58  | 1.87   | 1.45  | 1.54   | 1.91  | 1.85 | 2.40  | 2.89   | 2.2   | 2.13 | 2.17  | 2.2   | 2.17  | 2.16  | 3.62  | 3.2   |
| [S II] $\lambda$ 6716                      | 0.66  | 0.62   | 0.57  | 0.57   | 0.98  | 0.7  | 1.44  | 0.6    | 1.53  | 0.68 | 1.65  | 0.87  | 1.65  | 0.8   | 3.25  | 1.35  |
| [S II] $\lambda$ 6731                      | 0.54  | 0.8    | 0.48  | 0.95   | 0.66  | 1.4  | 0.88  | 1.0    | 0.80  | 1.0  | 0.8   | 1.1   | 0.8   | 1.0   | 1.46  | 2.    |
| FWHM(km s $^{-1}$ )                        | 0.0   | —      | 100   | —      | 200   | —    | 300   | —      | 400   | —    | 500   | —     | 600   | —     | 700   | —     |
| V $_s$ (km s $^{-1}$ )                     | —     | 60     | —     | 150    | —     | 220  | —     | 240    | —     | 440  | —     | 510   | —     | 600   | —     | 700   |
| n $_0$ (cm $^{-3}$ )                       | —     | 270    | —     | 250    | —     | 240  | —     | 310    | —     | 100  | —     | 60    | —     | 58    | —     | 70    |
| D(10 $^{18}$ cm)                           | —     | 0.0013 | —     | 0.001  | —     | 0.1  | —     | 0.1    | —     | 0.13 | —     | 0.13  | —     | 0.13  | —     | 0.08  |
| F (units $^1$ )                            | —     | 0.36   | —     | 0.74   | —     | 2.6  | —     | 2.6    | —     | 1.8  | —     | 0.7   | —     | 0.68  | —     | 1.5   |
| O/H (10 $^{-4}$ )                          | —     | 6.6    | —     | 6.6    | —     | 5.9  | —     | 6.1    | —     | 5.0  | —     | 6.6   | —     | 6.6   | —     | 6.6   |
| N/H (10 $^{-4}$ )                          | —     | 1.2    | —     | 1.2    | —     | 0.4  | —     | 0.6    | —     | 0.4  | —     | 0.5   | —     | 0.5   | —     | 0.1   |
| Ne/H(10 $^{-4}$ )                          | —     | 1.     | —     | 1.     | —     | 1.   | —     | 1.     | —     | 1.   | —     | 1.    | —     | 1.55  | —     | 1.4   |
| S/H (10 $^{-4}$ )                          | —     | 0.6    | —     | 1.     | —     | 0.08 | —     | 0.08   | —     | 0.08 | —     | 0.1   | —     | 0.1   | —     | 0.3   |
| H $\beta$ (erg)                            | —     | 3.5e-4 | —     | 6.4e-4 | —     | 0.05 | —     | 0.0564 | —     | 0.04 | —     | 0.014 | —     | 0.015 | —     | 0.036 |

$^1$  in  $10^{10}$  phot cm $^{-2}$ s $^{-1}$ eV $^{-1}$  at the Lyman limit ( $\alpha_{UV} = -1.5$ ,  $\alpha_X = -0.7$ );

**Table C8:** Simulation for  $V < 0$  of the CN region of IC 5063. For each bin there are the observed quantities and the results of the models. The first nine rows show the comparison between the observed and the synthetic spectra, the remaining rows show the input parameters of each model.

| line                                       | bin -1 |      | bin -2 |      | bin -3 |      | bin -4 |       | bin -5 |      | bin -6 |       | bin -7    |          |
|--------------------------------------------|--------|------|--------|------|--------|------|--------|-------|--------|------|--------|-------|-----------|----------|
|                                            | obs.   | mod. | obs.   | mod. | obs.   | mod. | obs.   | mod.  | obs.   | mod. | obs.   | mod.  | obs.      | mod.     |
| [O II] $\lambda$ 3727+                     | 3.76   | 3.7  | 3.9    | 3.6  | 2.5    | 2.6  | 2.3    | 2.48  | 2.00   | 2.17 | 3.15   | 3.13  | 0. + 0.43 | 1. + 0.5 |
| [Ne III] $\lambda$ 3869+                   | 1.78   | 1.77 | 1.68   | 1.57 | 1.5    | 1.56 | 1.34   | 1.6   | 1.5    | 1.5  | 3.05   | 2.5   | 1.3       | 1.4      |
| [He II] $\lambda$ 4686                     | 0.2    | 0.3  | 0.15   | 0.27 | 0.1    | 0.25 | 0.025  | 0.28  | 0.0    | 0.26 | 0.0    | 0.36  | 0.0       | 0.3      |
| [O III] $\lambda$ 5007+                    | 11.6   | 11.8 | 9.57   | 9.76 | 9.8    | 9.6  | 10.41  | 10.67 | 9.84   | 9.84 | 12.1   | 12.3  | 8.67      | 8.6      |
| [O I] $\lambda$ 6300,[S II] $\lambda$ 6310 | 0.32   | 0.55 | 0.39   | 0.47 | 0.47   | 0.5  | 0.44   | 0.5   | 0.46   | 0.45 | 0.4    | 0.4   | 0.4       | 0.4      |
| H $\alpha$                                 | 2.86   | 2.98 | 2.86   | 2.99 | 2.86   | 3.0  | 2.86   | 3.0   | 2.86   | 3.0  | 2.86   | 2.97  | 2.86      | 2.98     |
| [N II] $\lambda$ 6584                      | 1.7    | 1.99 | 2.0    | 2.13 | 2.36   | 2.34 | 2.42   | 2.5   | 2.3    | 2.3  | 2.72   | 2.7   | 1.56      | 1.89     |
| [S II] $\lambda$ 6716                      | 0.73   | 0.57 | 0.83   | 0.4  | 0.97   | 0.4  | 1.     | 0.4   | 0.89   | 0.3  | 0.88   | 0.4   | 0.9       | 0.5      |
| [S II] $\lambda$ 6731                      | 0.45   | 0.82 | 0.34   | 0.67 | 0.37   | 0.7  | 0.46   | 0.7   | 0.37   | 0.6  | 0.47   | 0.74  | 1.0       | 1.0      |
| FWHM(km s <sup>-1</sup> )                  | -100   | —    | -200   | —    | -300   | —    | -400   | —     | -500   | —    | -600   | —     | -700      | —        |
| V <sub>s</sub> (km s <sup>-1</sup> )       | —      | 100  | —      | 200  | —      | 300  | —      | 400   | —      | 500  | —      | 600   | —         | 700      |
| n <sub>0</sub> (cm <sup>-3</sup> )         | —      | 480  | —      | 420  | —      | 420  | —      | 290   | —      | 260  | —      | 200   | —         | 200      |
| D(10 <sup>18</sup> cm)                     | —      | 0.68 | —      | 0.68 | —      | 0.68 | —      | 0.05  | —      | 0.05 | —      | 0.047 | —         | 0.042    |
| F (units <sup>1</sup> )                    | —      | 5.   | —      | 5.   | —      | 10.  | —      | 11.   | —      | 12.2 | —      | 17.   | —         | 19.      |
| O/H (10 <sup>-4</sup> )                    | —      | 6.   | —      | 6.6  | —      | 6.6  | —      | 6.4   | —      | 6.4  | —      | 6.5   | —         | 6.6      |
| N/H (10 <sup>-4</sup> )                    | —      | 0.5  | —      | 0.5  | —      | 0.6  | —      | 0.7   | —      | 0.7  | —      | 0.7   | —         | 0.7      |
| Ne/H(10 <sup>-4</sup> )                    | —      | 1.   | —      | 1.   | —      | 1.   | —      | 1.    | —      | 1.   | —      | 1.5   | —         | 1.3      |
| S/H (10 <sup>-4</sup> )                    | —      | 0.04 | —      | 0.06 | —      | 0.07 | —      | 0.1   | —      | 0.1  | —      | 0.14  | —         | 0.3      |
| H $\beta$ (erg)                            | —      | 0.09 | —      | 0.1  | —      | 0.21 | —      | 0.24  | —      | 0.29 | —      | 0.33  | —         | 0.5      |

<sup>1</sup> in 10<sup>10</sup> phot cm<sup>-2</sup>s<sup>-1</sup>eV<sup>-1</sup> at the Lyman limit ( $\alpha_{UV} = -1.5$ ,  $\alpha_X = -0.7$ );

**Table C9:** Simulation for  $v \geq 0$  of the CS region of IC 5063. For each bin there are the observed quantities and the results of the models. The first nine rows show the comparison between the observed and the synthetic spectra, the remaining rows show the input parameters of each model.

|                                            | bin 0 |       | bin 1 |                    | bin 2 |                    | bin 3 |                      | bin 4 |       | bin 5 |      | bin 6 |      |
|--------------------------------------------|-------|-------|-------|--------------------|-------|--------------------|-------|----------------------|-------|-------|-------|------|-------|------|
| line                                       | obs.  | mod.  | obs.  | mod.               | obs.  | mod.               | obs.  | mod.                 | obs.  | mod.  | obs.  | mod. | obs.  | mod. |
| [O II] $\lambda$ 3727+                     | 2.7   | 2.4   | 3.13  | 3.2                | 4.72  | 4.9                | 4.33  | 4.0                  | 5.5   | 5.6   | 2.29  | 2.6  | 7.4   | 7.   |
| [Ne III] $\lambda$ 3869+                   | 1.31  | 1.37  | 1.48  | 1.23               | 1.9   | 1.6                | 2.17  | 1.17                 | 2.5   | 2.16  | 1.22  | 1.5  | 4.7   | 3.7  |
| [He II] $\lambda$ 4686                     | 0.18  | 0.45  | 0.17  | 0.32               | 0.18  | 0.21               | 0.13  | 0.26                 | 0.1   | 0.38  | 0.094 | 0.45 | 0.0   | 0.9  |
| [O III] $\lambda$ 5007+                    | 13.6  | 13.8  | 13.42 | 12.8               | 12.34 | 12.36              | 10.82 | 10.2                 | 12.12 | 12.13 | 12.43 | 12.2 | 25.7  | 24.3 |
| [O I] $\lambda$ 6300,[S II] $\lambda$ 6310 | 0.27  | 0.35  | 0.34  | 0.3                | 0.45  | 0.37               | 0.5   | 0.3                  | 0.34  | 0.6   | 0.74  | 1.0  | 0.44  | 0.44 |
| H $\alpha$                                 | 2.86  | 2.95  | 2.86  | 3.3                | 2.86  | 3.4                | 2.86  | 3.2                  | 2.86  | 2.98  | 2.69  | 3.   | 2.5   | 3.8  |
| [N II] $\lambda$ 6584                      | 1.58  | 1.36  | 1.56  | 1.58               | 2.03  | 1.9                | 1.97  | 2.13                 | 2.32  | 2.0   | 4.44  | 4.2  | 14.1  | 11.  |
| [S II] $\lambda$ 6716                      | 0.65  | 0.6   | 0.62  | 0.64               | 0.9   | 0.87               | 0.82  | 0.95                 | 0.66  | 0.61  | 0.48  | 0.43 | 0.31  | 0.24 |
| [S II] $\lambda$ 6731                      | 0.64  | 0.75  | 0.59  | 1.0                | 0.79  | 1.3                | 0.73  | 1.58                 | 0.80  | 0.76  | 1.49  | 0.8  | 4.4   | 0.5  |
| FWHM(km s $^{-1}$ )                        | 0.0   | —     | 100   | —                  | 200   | —                  | 300   | —                    | 400   | —     | 500   | —    | 600   | —    |
| V $_s$ (km s $^{-1}$ )                     | —     | 60    | —     | 150                | —     | 180                | —     | 300                  | —     | 410   | —     | 500  | —     | 600  |
| n $_0$ (cm $^{-3}$ )                       | —     | 320   | —     | 220                | —     | 180                | —     | 140                  | —     | 70    | —     | 220  | —     | 210  |
| D(10 $^{18}$ cm)                           | —     | 1.0   | —     | 0.001              | —     | 0.002              | —     | 0.007                | —     | 1.    | —     | 0.1  | —     | 0.17 |
| F (units $^1$ )                            | —     | 1.0   | —     | 0.6                | —     | 0.32               | —     | 0.4                  | —     | 1.5   | —     | 16.  | —     | 253. |
| O/H (10 $^{-4}$ )                          | —     | 5.8   | —     | 6.6                | —     | 6.4                | —     | 6.7                  | —     | 5.2   | —     | 6.9  | —     | 7.   |
| N/H (10 $^{-4}$ )                          | —     | 0.7   | —     | 1.2                | —     | 1.2                | —     | 1.2                  | —     | 0.7   | —     | 0.9  | —     | 2.2  |
| Ne/H(10 $^{-4}$ )                          | —     | 1.    | —     | 1.                 | —     | 1.                 | —     | 1.                   | —     | 1.    | —     | 1.2  | —     | 1.   |
| S/H (10 $^{-4}$ )                          | —     | 0.04  | —     | 1.                 | —     | 1.                 | —     | 1.                   | —     | 0.04  | —     | 0.1  | —     | 0.3  |
| H $\beta$ (erg)                            | —     | 0.136 | —     | $7 \times 10^{-4}$ | —     | $5 \times 10^{-4}$ | —     | $9.2 \times 10^{-4}$ | —     | 0.023 | —     | 0.3  | —     | 2.59 |

$^1$  in  $10^{10}$  phot cm $^{-2}$ s $^{-1}$ eV $^{-1}$  at the Lyman limit ( $\alpha_{UV} = -1.5$ ,  $\alpha_X = -0.7$ );

**Table C10:** Simulation for  $v < 0$  of the CS region of IC 5063. For each bin there are the observed quantities and the results of the models. The first nine rows show the comparison between the observed and the synthetic spectra, the remaining rows show the input parameters of each model.

| line                                       | bin 1 |                      | bin 2 |                      | bin 3 |                    | bin 4 |       |
|--------------------------------------------|-------|----------------------|-------|----------------------|-------|--------------------|-------|-------|
|                                            | obs.  | mod.                 | obs.  | mod.                 | obs.  | mod.               | obs.  | mod.  |
| [O II] $\lambda$ 3727+                     | 2.65  | 2.8                  | 3.14  | 3.2                  | 5.    | 5.2                | 7.8   | 8.3   |
| [Ne III] $\lambda$ 3869+                   | 1.58  | 1.3                  | 1.31  | 1.13                 | 1.37  | 1.47               | 0.59  | 1.3   |
| [He II] $\lambda$ 4686                     | 0.17  | 0.4                  | 0.08  | 0.3                  | 0.0   | 0.23               | 0.0   | 0.5   |
| [O III] $\lambda$ 5007+                    | 14.67 | 14.89                | 11.6  | 11.3                 | 11.5  | 11.9               | 14.63 | 14.7  |
| [O I] $\lambda$ 6300,[S II] $\lambda$ 6310 | 0.36  | 0.34                 | 0.34  | 0.3                  | 0.45  | 0.37               | 0.94  | 1.    |
| H $\alpha$                                 | 2.86  | 3.3                  | 2.86  | 3.2                  | 2.86  | 3.3                | 2.86  | 3.    |
| [N II] $\lambda$ 6584                      | 1.73  | 1.37                 | 1.98  | 1.6                  | 3.    | 2.6                | 8.67  | 7.    |
| [S II] $\lambda$ 6716                      | 0.8   | 0.6                  | 0.95  | 0.8                  | 1.    | 1.1                | 1.7   | 1.1   |
| [S II] $\lambda$ 6731                      | 0.76  | 1.88                 | 0.85  | 1.16                 | 0.72  | 1.8                | 1.2   | 1.2   |
| FWHM(km s $^{-1}$ )                        | -100  | —                    | -200  | —                    | -300  | —                  | -400  | —     |
| $V_s$ (km s $^{-1}$ )                      | —     | 150                  | —     | 200                  | —     | 300                | —     | 410   |
| $n_0$ (cm $^{-3}$ )                        | —     | 220                  | —     | 140                  | —     | 140                | —     | 50    |
| D(10 $^{18}$ cm)                           | —     | 0.001                | —     | 0.004                | —     | 0.007              | —     | 0.7   |
| F (units $^1$ )                            | —     | 0.8                  | —     | 0.42                 | —     | 0.33               | —     | 2.1   |
| O/H (10 $^{-4}$ )                          | —     | 6.6                  | —     | 6.4                  | —     | 6.6                | —     | 5.5   |
| N/H (10 $^{-4}$ )                          | —     | 1.2                  | —     | 1.2                  | —     | 1.3                | —     | 1.2   |
| Ne/H(10 $^{-4}$ )                          | —     | 1.                   | —     | 1.                   | —     | 1.                 | —     | 0.5   |
| S/H (10 $^{-4}$ )                          | —     | 1.                   | —     | 1.                   | —     | 1.                 | —     | 0.1   |
| H $\beta$ (erg)                            | —     | $6.6 \times 10^{-4}$ | —     | $6.3 \times 10^{-4}$ | —     | $7 \times 10^{-4}$ | —     | 0.029 |

$^1$  in  $10^{10}$  phot cm $^{-2}$ s $^{-1}$ eV $^{-1}$  at the Lyman limit ( $\alpha_{UV} = -1.5$ ,  $\alpha_X = -0.7$ );

**Table C11:** Simulation for  $v \geq 0$  of the S0 region of IC 5063. For each bin there are the observed quantities and the results of the models. The first nine rows show the comparison between the observed and the synthetic spectra, the remaining rows show the input parameters of each model.

| line                                       | bin 0 |       | bin 1 |      | bin 2 |      | bin 3 |       | bin 4 |       | bin 5 |       |
|--------------------------------------------|-------|-------|-------|------|-------|------|-------|-------|-------|-------|-------|-------|
|                                            | obs.  | mod.  | obs.  | mod. | obs.  | mod. | obs.  | mod.  | obs.  | mod.  | obs.  | mod.  |
| [O II] $\lambda$ 3727+                     | 2.37  | 2.4   | 2.52  | 3.0  | 2.98  | 2.6  | 3.23  | 2.9   | 2.3   | 2.8   | 2.07  | 2.5   |
| [Ne III] $\lambda$ 3869+                   | 1.4   | 1.34  | 1.46  | 2.0  | 1.59  | 2.0  | 1.9   | 1.7   | 2.7   | 2.4   | 1.5   | 1.6   |
| [He II] $\lambda$ 4686                     | 0.16  | 0.44  | 0.2   | 0.4  | 0.2   | 0.38 | 0.22  | 0.3   | 0.21  | 0.35  | 0.25  | 0.4   |
| [O III] $\lambda$ 5007+                    | 13.2  | 13.3  | 13.85 | 13.5 | 14.0  | 14.0 | 13.2  | 13.67 | 14.4  | 14.46 | 15.4  | 14.6  |
| [O I] $\lambda$ 6300,[S II] $\lambda$ 6310 | 0.33  | 0.33  | 0.35  | 0.7  | 0.37  | 0.7  | 0.28  | 0.3   | 0.27  | 0.21  | 0.5   | 0.2   |
| H $\alpha$                                 | 2.87  | 2.98  | 2.86  | 3.0  | 2.86  | 3.0  | 2.86  | 2.9   | 2.86  | 2.89  | 2.86  | 2.88  |
| [N II] $\lambda$ 6584                      | 1.84  | 1.5   | 1.88  | 2.0  | 1.86  | 1.98 | 1.65  | 1.76  | 1.74  | 1.77  | 2.23  | 1.9   |
| [S II] $\lambda$ 6716                      | 1.5   | 0.7   | 0.83  | 0.6  | 0.69  | 0.44 | 0.49  | 0.38  | 0.44  | 0.35  | 0.42  | 0.47  |
| [S II] $\lambda$ 6731                      | 0.7   | 0.93  | 0.76  | 0.86 | 0.68  | 0.74 | 0.58  | 0.8   | 0.63  | 0.75  | 0.77  | 1.0   |
| FWHM(km s $^{-1}$ )                        | 0.0   | —     | 100   | —    | 200   | —    | 300   | —     | 400   | —     | 500   | —     |
| V <sub>s</sub> (km s $^{-1}$ )             | —     | 60    | —     | 100  | —     | 180  | —     | 290   | —     | 400   | —     | 500   |
| n <sub>0</sub> (cm $^{-3}$ )               | —     | 320   | —     | 620  | —     | 620  | —     | 430   | —     | 340   | —     | 300   |
| D(10 $^{18}$ cm)                           | —     | 1.0   | —     | 0.7  | —     | 0.5  | —     | 0.008 | —     | 0.01  | —     | 0.012 |
| F (units $^1$ )                            | —     | 0.95  | —     | 11.  | —     | 23.  | —     | 10.   | —     | 12.   | —     | 15.   |
| O/H (10 $^{-4}$ )                          | —     | 5.8   | —     | 5.8  | —     | 6.6  | —     | 6.6   | —     | 6.1   | —     | 6.5   |
| N/H (10 $^{-4}$ )                          | —     | 0.8   | —     | 0.7  | —     | 0.5  | —     | 0.5   | —     | 0.5   | —     | 0.6   |
| Ne/H(10 $^{-4}$ )                          | —     | 1.    | —     | 1.   | —     | 1.   | —     | 1.    | —     | 1.3   | —     | 1.0   |
| S/H (10 $^{-4}$ )                          | —     | 0.05  | —     | 0.04 | —     | 0.06 | —     | 0.18  | —     | 0.18  | —     | 0.3   |
| H $\beta$ (erg)                            | —     | 0.135 | —     | 0.17 | —     | 0.35 | —     | 0.19  | —     | 0.2   | —     | 0.3   |

<sup>1</sup> in 10 $^{10}$  phot cm $^{-2}$ s $^{-1}$ eV $^{-1}$  at the Lyman limit ( $\alpha_{UV} = -1.5$ ,  $\alpha_X = -0.7$ );

**Table C12:** Simulation for  $v < 0$  of the S0 region of IC 5063 For each bin there are the observed quantities and the results of the models. The first nine rows show the comparison between the observed and the synthetic spectra, the remaining rows show the input parameters of each model.

|                                            | bin 1 |       | bin 2 |       | bin 3 |       | bin 4 |       |
|--------------------------------------------|-------|-------|-------|-------|-------|-------|-------|-------|
| line                                       | obs.  | mod.  | obs.  | mod.  | obs.  | mod.  | obs.  | mod.  |
| [O II] $\lambda$ 3727+                     | 2.43  | 2.68  | 3.06  | 2.8   | 3.58  | 3.5   | 5.43  | 5.47  |
| [Ne III] $\lambda$ 3869+                   | 1.27  | 1.4   | 1.35  | 1.6   | 2.2   | 1.6   | 0.12  | 1.0   |
| [He II] $\lambda$ 4686                     | 0.15  | 0.37  | 0.12  | 0.3   | 0.02  | 0.28  | 0.0   | 0.2   |
| [O III] $\lambda$ 5007+                    | 12.97 | 13.0  | 12.0  | 12.0  | 11.4  | 11.1  | 8.98  | 8.88  |
| [O I] $\lambda$ 6300,[S II] $\lambda$ 6310 | 0.32  | 0.46  | 0.3   | 0.3   | 0.41  | 0.46  | 0.53  | 0.4   |
| H $\alpha$                                 | 2.86  | 2.9   | 2.86  | 2.9   | 2.86  | 2.9   | 2.86  | 2.96  |
| [N II] $\lambda$ 6584                      | 1.9   | 1.9   | 2.07  | 2.2   | 2.18  | 2.    | 3.22  | 3.86  |
| [S II] $\lambda$ 6716                      | 0.9   | 0.53  | 1.09  | 0.54  | 0.92  | 0.5   | 0.98  | 0.82  |
| [S II] $\lambda$ 6731                      | 0.8   | 1.1   | 0.9   | 1.1   | 1.0   | 1.0   | 0.72  | 1.3   |
| FWHM(km s $^{-1}$ )                        | -100  | —     | -200  | —     | -300  | —     | -400  | —     |
| V $_s$ (km s $^{-1}$ )                     | —     | 100   | —     | 170   | —     | 300   | —     | 400   |
| n $_0$ (cm $^{-3}$ )                       | —     | 850   | —     | 600   | —     | 370   | —     | 130   |
| D(10 $^{18}$ cm)                           | —     | 0.007 | —     | 0.01  | —     | 0.008 | —     | 0.08  |
| F (units $^1$ )                            | —     | 9.2   | —     | 7.    | —     | 6.    | —     | 2.2   |
| O/H (10 $^{-4}$ )                          | —     | 5.    | —     | 6.6   | —     | 6.6   | —     | 6.1   |
| N/H (10 $^{-4}$ )                          | —     | 0.5   | —     | 0.6   | —     | 0.5   | —     | 0.8   |
| Ne/H(10 $^{-4}$ )                          | —     | 0.7   | —     | 1.    | —     | 1.    | —     | 0.7   |
| S/H (10 $^{-4}$ )                          | —     | 0.2   | —     | 0.2   | —     | 0.18  | —     | 0.12  |
| H $\beta$ (erg)                            | —     | 0.14  | —     | 0.168 | —     | 0.12  | —     | 0.054 |

$^1$  in 10 $^{10}$  phot cm $^{-2}$ s $^{-1}$ eV $^{-1}$  at the Lyman limit ( $\alpha_{UV} = -1.5$ ,  $\alpha_X = -0.7$ );

**Table C13:** Simulation for  $v \geq 0$  of the S1 region of IC 5063. For each bin there are the observed quantities and the results of the models. The first nine rows show the comparison between the observed and the synthetic spectra, the remaining rows show the input parameters of each model.

| line                                       | bin 0 |        | bin 1 |      | bin 2 |      | bin 3 |       | bin 4 |       | bin 5 |      | bin 6 |      |
|--------------------------------------------|-------|--------|-------|------|-------|------|-------|-------|-------|-------|-------|------|-------|------|
|                                            | obs.  | mod.   | obs.  | mod. | obs.  | mod. | obs.  | mod.  | obs.  | mod.  | obs.  | mod. | obs.  | mod. |
| [O II] $\lambda$ 3727+                     | 3.26  | 3.0    | 2.5   | 2.86 | 2.88  | 3.1  | 4.7   | 4.2   | 6.3   | 6.8   | 13.9  | 12.2 | 19.   | 18.  |
| [Ne III] $\lambda$ 3869+                   | 1.7   | 1.3    | 1.6   | 1.8  | 1.7   | 1.7  | 2.6   | 2.1   | 3.3   | 3.0   | 4.9   | 3.9  | 1.4   | 3.   |
| [He II] $\lambda$ 4686                     | 0.15  | 0.4    | 0.2   | 0.44 | 0.22  | 0.4  | 0.22  | 0.34  | 0.12  | 0.9   | 0.0   | 0.84 | 0.0   | 0.6  |
| [O III] $\lambda$ 5007+                    | 13.22 | 13.2   | 14.64 | 14.7 | 14.65 | 14.5 | 12.54 | 13.0  | 14.0  | 13.86 | 17.7  | 17.0 | 19.97 | 19   |
| [O I] $\lambda$ 6300,[S II] $\lambda$ 6310 | 0.29  | 0.2    | 0.33  | 0.7  | 0.32  | 0.7  | 0.24  | 0.7   | 0.29  | 1.0   | 0.25  | 0.4  | 0.04  | 0.2  |
| H $\alpha$                                 | 2.87  | 3.0    | 2.86  | 3.0  | 2.86  | 3.0  | 2.86  | 3.0   | 2.86  | 3.8   | 2.86  | 3.4  | 2.86  | 3.5  |
| [N II] $\lambda$ 6584                      | 1.82  | 1.85   | 1.7   | 2.0  | 1.6   | 1.97 | 1.49  | 2.3   | 1.71  | 2.8   | 2.3   | 2.77 | 1.87  | 2.7  |
| [S II] $\lambda$ 6716                      | 0.77  | 0.62   | 0.82  | 0.6  | 0.59  | 0.33 | 0.4   | 0.38  | 0.31  | 0.46  | 0.6   | 0.5  | 0.8   | 0.7  |
| [S II] $\lambda$ 6731                      | 0.7   | 0.8    | 0.69  | 0.8  | 0.55  | 0.55 | 0.5   | 0.6   | 0.56  | 0.87  | 0.97  | 1.0  | 0.7   | 1.   |
| FWHM(km s $^{-1}$ )                        | 0.0   | —      | 100   | —    | 200   | —    | 300   | —     | 400   | —     | 500   | —    | 600   | —    |
| V <sub>s</sub> (km s $^{-1}$ )             | —     | 60     | —     | 90   | —     | 200  | —     | 320   | —     | 430   | —     | 510  | —     | 600  |
| n <sub>0</sub> (cm $^{-3}$ )               | —     | 270    | —     | 810  | —     | 420  | —     | 250   | —     | 230   | —     | 150  | —     | 80   |
| D(10 $^{18}$ cm)                           | —     | 0.0013 | —     | 0.5  | —     | 0.22 | —     | 0.6   | —     | 0.13  | —     | 0.3  | —     | 0.92 |
| F (units $^1$ )                            | —     | 0.36   | —     | 15.  | —     | 18.  | —     | 11.   | —     | 70.   | —     | 90.  | —     | 65.  |
| O/H (10 $^{-4}$ )                          | —     | 6.6    | —     | 5.8  | —     | 6.6  | —     | 6.6   | —     | 6.5   | —     | 6.9  | —     | 7.1  |
| N/H (10 $^{-4}$ )                          | —     | 1.2    | —     | 0.5  | —     | 0.5  | —     | 0.5   | —     | 0.4   | —     | 1.2  | —     | 0.4  |
| Ne/H(10 $^{-4}$ )                          | —     | 1.2    | —     | 0.8  | —     | 0.8  | —     | 1.    | —     | 1.0   | —     | 1.2  | —     | 1.   |
| S/H (10 $^{-4}$ )                          | —     | 0.6    | —     | 0.04 | —     | 0.04 | —     | 0.04  | —     | 0.2   | —     | 0.4  | —     | 0.3  |
| H $\beta$ (erg)                            | —     | 3.5e-4 | —     | 0.21 | —     | 0.26 | —     | 0.166 | —     | 0.6   | —     | 1.16 | —     | 0.79 |

$^1$  in  $10^{10}$  phot cm $^{-2}$ s $^{-1}$ eV $^{-1}$  at the Lyman limit ( $\alpha_{UV} = -1.5$ ,  $\alpha_X = -0.7$ );

**Table C14:** Simulation for  $V < 0$  of the S1 region of IC 5063. For each bin there are the observed quantities and the results of the models. The first nine rows show the comparison between the observed and the synthetic spectra, the remaining rows show the input parameters of each model.

|                                            | bin 1 |       | bin 2 |      | bin 3 |       | bin 4 |                      |
|--------------------------------------------|-------|-------|-------|------|-------|-------|-------|----------------------|
| line                                       | obs.  | mod.  | obs.  | mod. | obs.  | mod.  | obs.  | mod.                 |
| [O II] $\lambda$ 3727+                     | 3.1   | 2.93  | 3.88  | 3.7  | 6.06  | 6.3   | 284.4 | 70.                  |
| [Ne III] $\lambda$ 3869+                   | 1.55  | 1.55  | 1.55  | 1.4  | 1.81  | 2.0   | —     | —                    |
| [He II] $\lambda$ 4686                     | 0.14  | 0.37  | 0.09  | 0.3  | 0.0   | 0.3   | 0.0   | —                    |
| [O III] $\lambda$ 5007+                    | 12.5  | 12.55 | 11.7  | 11.7 | 8.57  | 8.8   | 23.55 | 42.                  |
| [O I] $\lambda$ 6300,[S II] $\lambda$ 6310 | 0.24  | 0.6   | 0.23  | 0.5  | 0.28  | 2.0   | 0.31  | 0.2                  |
| H $\alpha$                                 | 2.86  | 3.0   | 2.86  | 2.97 | 2.86  | 3.0   | 2.86  | 5.9                  |
| [N II] $\lambda$ 6584                      | 1.87  | 2.0   | 1.95  | 2.1  | 1.98  | 1.8   | 2.8   | 2.                   |
| [S II] $\lambda$ 6716                      | 0.8   | 0.5   | 0.9   | 0.5  | 0.75  | 0.97  | 0.48  | 0.4                  |
| [S II] $\lambda$ 6731                      | 0.73  | 0.74  | 0.84  | 0.84 | 0.96  | 1.07  | 0.37  | 0.3                  |
| FWHM(km s $^{-1}$ )                        | −100  | —     | −200  | —    | −300  | —     | −400  | —                    |
| V $_s$ (km s $^{-1}$ )                     | —     | 96    | —     | 200  | —     | 300   | —     | 400                  |
| n $_0$ (cm $^{-3}$ )                       | —     | 760   | —     | 400  | —     | 130   | —     | 20                   |
| D(10 $^{18}$ cm)                           | —     | 0.5   | —     | 0.22 | —     | 3.    | —     | 0.186                |
| F (units $^1$ )                            | —     | 9.5   | —     | 6.   | —     | 1.2   | —     | 0.0                  |
| O/H (10 $^{-4}$ )                          | —     | 5.8   | —     | 6.6  | —     | 6.5   | —     | 6.5                  |
| N/H (10 $^{-4}$ )                          | —     | 0.5   | —     | 0.5  | —     | 0.3   | —     | 0.2                  |
| Ne/H(10 $^{-4}$ )                          | —     | 0.8   | —     | 0.8  | —     | 0.8   | —     | 0.1                  |
| S/H (10 $^{-4}$ )                          | —     | 0.04  | —     | 0.06 | —     | 0.04  | —     | 0.01                 |
| H $\beta$ (erg)                            | —     | 0.16  | —     | 0.11 | —     | 0.026 | —     | $2.6 \times 10^{-5}$ |

$^1$  in  $10^{10}$  phot cm $^{-2}$ s $^{-1}$ eV $^{-1}$  at the Lyman limit ( $\alpha_{UV} = -1.5$ ,  $\alpha_X = -0.7$ );



**Table C15:** Simulation for  $V \geq 0$  of the S2 region of IC 5063. For each bin there are the observed quantities and the results of the models. The first nine rows show the comparison between the observed and the synthetic spectra, the remaining rows show the input parameters of each model.

| line                                       | bin 0 |                      | bin 1 |            | bin 2 |       | bin 3 |      |
|--------------------------------------------|-------|----------------------|-------|------------|-------|-------|-------|------|
|                                            | obs.  | mod.                 | obs.  | mod.       | obs.  | mod.  | obs.  | mod. |
| [O II] $\lambda$ 3727+                     | 2.54  | 2.4                  | 2.38  | 2.5        | 2.6   | 2.8   | 2.53  | 2.0  |
| [Ne III] $\lambda$ 3869+                   | 1.87  | 1.3                  | 1.6   | 1.5        | 1.9   | 2.4   | 1.5   | 1.75 |
| [He II] $\lambda$ 4686                     | 0.09  | 0.4                  | 0.15  | 0.49       | 0.19  | 0.5   | 0.05  | 0.28 |
| [O III] $\lambda$ 5007+                    | 11.0  | 11.7                 | 14.2  | 14.2       | 16.15 | 16.16 | 11.0  | 11.5 |
| [O I] $\lambda$ 6300,[S II] $\lambda$ 6310 | 0.25  | 0.2                  | 0.3   | 0.24       | 0.36  | 0.7   | 0.3   | 0.6  |
| H $\alpha$                                 | 2.86  | 3.0                  | 2.86  | 3.0        | 2.86  | 3.1   | 2.86  | 3.0  |
| [N II] $\lambda$ 6584                      | 1.74  | 1.64                 | 1.66  | 1.4        | 1.66  | 2.1   | 1.3   | 1.7  |
| [S II] $\lambda$ 6716                      | 0.87  | 0.6                  | 0.87  | 0.53       | 0.87  | 0.37  | 0.3   | 0.3  |
| [S II] $\lambda$ 6731                      | 0.69  | 0.7                  | 0.65  | 0.75       | 0.55  | 0.67  | 0.4   | 0.5  |
| FWHM(km s $^{-1}$ )                        | 0.0   | —                    | 100   | —          | 200   | —     | 300   | —    |
| V <sub>s</sub> (km s $^{-1}$ )             | —     | 55                   | —     | 100        | —     | 200   | —     | 300  |
| n <sub>0</sub> (cm $^{-3}$ )               | —     | 270                  | —     | 220        | —     | 520   | —     | 520  |
| D(10 $^{18}$ cm)                           | —     | 0.0015               | —     | 0.0014     | —     | 0.1   | —     | 0.1  |
| F (units $^1$ )                            | —     | 0.34                 | —     | 0.6        | —     | 33.   | —     | 23.  |
| O/H (10 $^{-4}$ )                          | —     | 6.6                  | —     | 6.6        | —     | 6.6   | —     | 6.6  |
| N/H (10 $^{-4}$ )                          | —     | 1.2                  | —     | 1.2        | —     | 0.5   | —     | 0.5  |
| Ne/H(10 $^{-4}$ )                          | —     | 1.4                  | —     | 1.4        | —     | 1.0   | —     | 1.0  |
| S/H (10 $^{-4}$ )                          | —     | 0.6                  | —     | 0.8        | —     | 0.06  | —     | 0.06 |
| H $\beta$ (erg)                            | —     | $3.2 \times 10^{-4}$ | —     | $6.6e - 4$ | —     | 0.39  | —     | 0.44 |

<sup>1</sup> in 10 $^{10}$  phot cm $^{-2}$ s $^{-1}$ eV $^{-1}$  at the Lyman limit ( $\alpha_{UV} = -1.5$ ,  $\alpha_X = -0.7$ );

**Table C16:** Simulation for  $V < 0$  of the S2 region of IC 5063. For each bin there are the observed quantities and the results of the models. The first nine rows show the comparison between the observed and the synthetic spectra, the remaining rows show the input parameters of each model.

| line                                       | bin -1 |      | bin -2 |       | bin -3 |      |
|--------------------------------------------|--------|------|--------|-------|--------|------|
|                                            | obs.   | mod. | obs.   | mod.  | obs.   | mod. |
| [O II] $\lambda$ 3727+                     | 2.66   | 2.8  | 2.37   | 2.4   | 3.85   | 3.87 |
| [Ne III] $\lambda$ 3869+                   | 1.84   | 1.54 | 1.2    | 1.4   | 1.54   | 1.46 |
| [He II] $\lambda$ 4686                     | 0.09   | 0.3  | 0.0    | 0.2   | 0.0    | 0.2  |
| [O III] $\lambda$ 5007+                    | 10.2   | 10.2 | 7.36   | 7.33  | 7.1    | 7.3  |
| [O I] $\lambda$ 6300,[S II] $\lambda$ 6310 | 0.25   | 0.5  | 0.29   | 0.4   | 0.93   | 0.8  |
| H $\alpha$                                 | 2.86   | 3.0  | 2.86   | 2.98  | 2.86   | 2.95 |
| [N II] $\lambda$ 6584                      | 1.88   | 1.7  | 1.88   | 1.98  | 2.47   | 2.6  |
| [S II] $\lambda$ 6716                      | 0.69   | 0.66 | 0.69   | 0.5   | 0.57   | 0.4  |
| [S II] $\lambda$ 6731                      | 0.64   | 0.99 | 0.65   | 0.815 | 0.54   | 0.6  |
| FWHM(km s $^{-1}$ )                        | -100   | —    | -200   | —     | -300   | —    |
| $V_s$ (km s $^{-1}$ )                      | —      | 100  | —      | 200   | —      | 300  |
| $n_0$ (cm $^{-3}$ )                        | —      | 600  | —      | 600   | —      | 280  |
| D(10 $^{18}$ cm)                           | —      | 1.0  | —      | 0.2   | —      | 0.32 |
| F (units $^1$ )                            | —      | 6.9  | —      | 7.0   | —      | 3.2  |
| O/H (10 $^{-4}$ )                          | —      | 6.0  | —      | 6.0   | —      | 6.0  |
| N/H (10 $^{-4}$ )                          | —      | 0.5  | —      | 0.8   | —      | 1.   |
| Ne/H(10 $^{-4}$ )                          | —      | 1.0  | —      | 1.0   | —      | 1.   |
| S/H (10 $^{-4}$ )                          | —      | 0.06 | —      | 0.08  | —      | 0.05 |
| H $\beta$ (erg)                            | —      | 0.14 | —      | 0.16  | —      | 0.07 |

$^1$  in 10 $^{10}$  phot cm $^{-2}$ s $^{-1}$ eV $^{-1}$  at the Lyman limit ( $\alpha_{UV} = -1.5$ ,  $\alpha_X = -0.7$ );

## **2 NGC 7212**

**Table C17:** Simulations for  $V \geq 0$  of the N2 region of NGC 7212. For each bin there are the observed quantities and the results of the models. The first nine rows show the comparison between the observed and the synthetic spectra, the remaining rows show the input parameters of each model.

| line                                        | bin 0 |       | bin 1 |      | bin 2 |      | bin 3 |       | bin 4 |       |
|---------------------------------------------|-------|-------|-------|------|-------|------|-------|-------|-------|-------|
|                                             | obs.  | mod.  | obs.  | mod. | obs.  | mod. | obs.  | mod.  | obs.  | mod.  |
| [O II] $\lambda$ 3727+                      | 4.2   | 4.6   | 3.06  | 3.07 | 2.72  | 2.76 | 2.8   | 2.7   | 1.83  | 1.6   |
| [O III] $\lambda$ 5007+                     | 10.8  | 10.9  | 9.5   | 9.11 | 7.88  | 7.7  | 6.0   | 6.2   | 3.99  | 4.5   |
| [O I] $\lambda$ 6300+,[S II] $\lambda$ 6310 | 0.39  | 0.3   | 0.4   | 0.5  | 0.42  | 0.4  | 1.26  | 1.3   | 1.8   | 0.7   |
| H $\alpha$                                  | 2.86  | 2.9   | 2.86  | 3.0  | 2.86  | 3.0  | 2.12  | 3.0   | 1.05  | 3.4   |
| [N II] $\lambda$ 6584                       | 1.72  | 1.75  | 1.63  | 1.68 | 1.8   | 2.0  | 2.0   | 1.96  | 1.18  | 0.84  |
| [S II] $\lambda$ 6716                       | 0.93  | 0.9   | 0.85  | 0.69 | 0.87  | 0.6  | 1.11  | 0.7   | 1.03  | 0.5   |
| [S II] $\lambda$ 6731                       | 0.7   | 1.13  | 0.61  | 1.   | 0.62  | 1.   | 0.72  | 1.1   | 0.8   | 0.85  |
| FWHM(km s $^{-1}$ )                         | 0.0   | —     | 100   | —    | 200   | —    | 300   | —     | 400   | —     |
| V $_s$ (km s $^{-1}$ )                      | —     | 55    | —     | 100  | —     | 200  | —     | 300   | —     | 400   |
| n $_0$ (cm $^{-3}$ )                        | —     | 220   | —     | 580  | —     | 530  | —     | 430   | —     | 200   |
| D(10 $^{18}$ cm)                            | —     | 0.12  | —     | 0.95 | —     | 0.85 | —     | 0.85  | —     | 0.85  |
| F (units $^1$ )                             | —     | 0.25  | —     | 0.89 | —     | 4.0  | —     | 5.0   | —     | 2.5   |
| O/H (10 $^4$ )                              | —     | 6.6   | —     | 6.6  | —     | 6.6  | —     | 6.6   | —     | 6.6   |
| N/H (10 $^4$ )                              | —     | 0.6   | —     | 0.5  | —     | 0.5  | —     | 0.5   | —     | 0.5   |
| Ne/H(10 $^4$ )                              | —     | 1.    | —     | 1.2  | —     | 1.2  | —     | 1.2   | —     | 1.2   |
| S/H (10 $^4$ )                              | —     | 0.15  | —     | 0.07 | —     | 0.1  | —     | 0.12  | —     | 0.16  |
| H $\beta$ (erg)                             | —     | 0.019 | —     | 0.12 | —     | 0.14 | —     | 0.156 | —     | 0.255 |

$^1$  in  $10^{10}$  phot cm $^{-2}$ s $^{-1}$ eV $^{-1}$  at the Lyman limit ( $\alpha_{UV} = -1.5$ ,  $\alpha_X = -0.7$ );

**Table C18:** Simulations for  $V < 0$  of the N2 region of NGC 7212. For each bin there are the observed quantities and the results of the models. The first nine rows show the comparison between the observed and the synthetic spectra, the remaining rows show the input parameters of each model.

| line                                        | bin -1 |      | bin -2 |      | bin -3 |      |
|---------------------------------------------|--------|------|--------|------|--------|------|
|                                             | obs.   | mod. | obs.   | mod. | obs.   | mod. |
| [O II] $\lambda$ 3727+                      | 3.14   | 3.1  | 2.05   | 2.2  | 0.94   | 0.91 |
| [O III] $\lambda$ 5007+                     | 10.7   | 10.4 | 8.6    | 8.3  | 4.84   | 4.53 |
| [O I] $\lambda$ 6300+,[S II] $\lambda$ 6310 | 0.48   | 0.5  | —      | —    | 0.66   | 0.5  |
| H $\alpha$                                  | 2.86   | 3.   | 2.86   | 3.06 | 0.37   | 3.37 |
| [N II] $\lambda$ 6584                       | 2.     | 1.7  | 2.12   | 1.6  | 0.96   | 0.96 |
| [S II] $\lambda$ 6716                       | 1.04   | 0.76 | 1.2    | 1.1  | 0.1    | 0.24 |
| [S II] $\lambda$ 6731                       | 0.89   | 1.13 | 1.4    | 1.9  | 0.19   | 0.4  |
| FWHM(km s $^{-1}$ )                         | −100   | —    | −200   | —    | −300   | —    |
| V $_s$ (km s $^{-1}$ )                      | —      | 100  | —      | 200  | —      | 300  |
| n $_0$ (cm $^{-3}$ )                        | —      | 580  | —      | 600  | —      | 500  |
| D(10 $^{18}$ cm)                            | —      | 0.95 | —      | 0.92 | —      | 0.93 |
| F (units $^1$ )                             | —      | 6.0  | —      | 9    | —      | 18   |
| O/H (10 $^4$ )                              | —      | 6.6  | —      | 6.6  | —      | 6.6  |
| N/H (10 $^4$ )                              | —      | 0.5  | —      | 0.7  | —      | 1.0  |
| Ne/H(10 $^4$ )                              | —      | 1.2  | —      | 1.2  | —      | 1.2  |
| S/H (10 $^4$ )                              | —      | 0.07 | —      | 0.2  | —      | 0.1  |
| H $\beta$ (erg)                             | —      | 0.13 | —      | 0.2  | —      | 0.7  |

<sup>1</sup> in 10 $^{10}$  phot cm $^{-2}$ s $^{-1}$ eV $^{-1}$  at the Lyman limit ( $\alpha_{UV} = -1.5$ ,  $\alpha_X = -0.7$ );

**Table C19:** Simulations for  $V \geq 0$  of the N1 region of NGC 7212. For each bin there are the observed quantities and the results of the models. The first nine rows show the comparison between the observed and the synthetic spectra, the remaining rows show the input parameters of each model.

| line                                        | bin 0 |                      | bin 1 |       | bin 2 |       | bin 3 |      | bin 4 |      |
|---------------------------------------------|-------|----------------------|-------|-------|-------|-------|-------|------|-------|------|
|                                             | obs.  | mod.                 | obs.  | mod.  | obs.  | mod.  | obs.  | mod. | obs.  | mod. |
| [O II] $\lambda$ 3727+                      | 3.33  | 3.3                  | 3.85  | 3.6   | 4.10  | 4.37  | 4.49  | 4.32 | 4.28  | 4.36 |
| [Ne III] $\lambda$ 3869+                    | 1.3   | 1.34                 | 1.47  | 1.5   | 1.5   | 1.6   | 1.7   | 1.74 | 2.    | 1.54 |
| He II $\lambda$ 4686                        | 0.13  | 0.33                 | 0.18  | 0.4   | 0.15  | 0.3   | 0.0   | 0.26 | 0.0   | 0.22 |
| [O III] $\lambda$ 5007+                     | 10.75 | 10.7                 | 12.9  | 13.0  | 12.48 | 12.45 | 8.74  | 8.9  | 7.3   | 7.46 |
| [O I] $\lambda$ 6300+,[S II] $\lambda$ 6310 | 0.46  | 0.12                 | 0.54  | 0.13  | 0.5   | 0.6   | 0.35  | 0.5  | 0.63  | 0.7  |
| H $\alpha$                                  | 2.86  | 3.2                  | 2.86  | 2.9   | 2.86  | 2.95  | 2.86  | 2.99 | 2.38  | 2.94 |
| [N II] $\lambda$ 6584                       | 2.05  | 2.15                 | 1.95  | 2.4   | 1.86  | 2.0   | 2.2   | 2.1  | 2.08  | 1.7  |
| [S II] $\lambda$ 6716                       | 1.16  | 0.5                  | 1.06  | 0.85  | 0.75  | 0.5   | 1.18  | 0.5  | 0.7   | 0.42 |
| [S II] $\lambda$ 6731                       | 0.9   | 0.6                  | 0.73  | 1.1   | 0.6   | 0.9   | 0.91  | 0.93 | 0.66  | 0.78 |
| FWHM(km s $^{-1}$ )                         | 0.0   | —                    | 100   | —     | 200   | —     | 300   | —    | 400   | —    |
| $V_s$ (km s $^{-1}$ )                       | —     | 55                   | —     | 100   | —     | 200   | —     | 300  | —     | 400  |
| $n_0$ (cm $^{-3}$ )                         | —     | 270                  | —     | 170   | —     | 300   | —     | 320  | —     | 200  |
| D(10 $^{18}$ cm)                            | —     | 0.0015               | —     | 0.045 | —     | 0.03  | —     | 0.03 | —     | 0.02 |
| F (units $^1$ )                             | —     | 0.25                 | —     | 0.89  | —     | 4.0   | —     | 5.0  | —     | 2.5  |
| O/H (10 $^4$ )                              | —     | 6.6                  | —     | 6.6   | —     | 6.6   | —     | 6.6  | —     | 6.6  |
| N/H (10 $^4$ )                              | —     | 1.2                  | —     | 1.2   | —     | 0.5   | —     | 0.4  | —     | 0.4  |
| Ne/H(10 $^4$ )                              | —     | 1.4                  | —     | 1.4   | —     | 1.0   | —     | 1.0  | —     | 1.2  |
| S/H (10 $^4$ )                              | —     | 0.4                  | —     | 0.4   | —     | 0.1   | —     | 0.1  | —     | 0.1  |
| H $\beta$ (erg)                             | —     | $3.6 \times 10^{-4}$ | —     | 0.011 | —     | 0.07  | —     | 0.12 | —     | 0.06 |

<sup>1</sup> in 10 $^{10}$  phot cm $^{-2}$ s $^{-1}$ eV $^{-1}$  at the Lyman limit ( $\alpha_{UV} = -1.5$ ,  $\alpha_X = -0.7$ );

**Table C20:** Simulations for  $V < 0$  of the N1 region of NGC 7212. For each bin there are the observed quantities and the results of the models. The first nine rows show the comparison between the observed and the synthetic spectra, the remaining rows show the input parameters of each model.

| line                                        | bin -1 |                      | bin -2 |       | bin -3 |       |
|---------------------------------------------|--------|----------------------|--------|-------|--------|-------|
|                                             | obs.   | mod.                 | obs.   | mod.  | obs.   | mod.  |
| [O II] $\lambda$ 3727+                      | 2.85   | 2.76                 | 5.7    | 5.9   | 3.85   | 4.1   |
| [Ne III] $\lambda$ 3869+                    | 1.9    | 1.45                 | 2.84   | 2.8   | 3.4    | 2.2   |
| He II $\lambda$ 4686                        | 0.15   | 0.4                  | 0.27   | 0.47  | 0.0    | 0.4   |
| [O III] $\lambda$ 5007+                     | 11.    | 11.1                 | 13.8   | 14.   | 14.14  | 14.   |
| [O I] $\lambda$ 6300+,[S II] $\lambda$ 6310 | 0.37   | 0.22                 | 0.28   | 0.5   | 0.06   | 0.1   |
| H $\alpha$                                  | 2.86   | 3.0                  | 2.86   | 2.97  | 2.86   | 2.9   |
| [N II] $\lambda$ 6584                       | 2.1    | 1.73                 | 2.     | 2.7   | 2.37   | 2.2   |
| [S II] $\lambda$ 6716                       | 1.09   | 0.63                 | 1.     | 1.3   | 0.93   | 0.82  |
| [S II] $\lambda$ 6731                       | 0.96   | 0.85                 | 1.16   | 1.4   | 1.24   | 1.35  |
| FWHM(km s $^{-1}$ )                         | -100   | —                    | -200   | —     | -300   | —     |
| V $_s$ (km s $^{-1}$ )                      | —      | 90                   | —      | 200   | —      | 300   |
| n $_0$ (cm $^{-3}$ )                        | —      | 200                  | —      | 80    | —      | 140   |
| D(10 $^{18}$ cm)                            | —      | 0.0016               | —      | 0.48  | —      | 0.05  |
| F (units $^1$ )                             | —      | 0.37                 | —      | 1.1   | —      | 3.3   |
| O/H (10 $^4$ )                              | —      | 6.6                  | —      | 6.6   | —      | 6.6   |
| N/H (10 $^4$ )                              | —      | 1.4                  | —      | 1.2   | —      | 1.2   |
| Ne/H(10 $^4$ )                              | —      | 1.6                  | —      | 1.6   | —      | 1.6   |
| S/H (10 $^4$ )                              | —      | 0.8                  | —      | 0.1   | —      | 0.2   |
| H $\beta$ (erg)                             | —      | $5.2 \times 10^{-4}$ | —      | 0.015 | —      | 0.055 |

<sup>1</sup> in  $10^{10}$  phot cm $^{-2}$ s $^{-1}$ eV $^{-1}$  at the Lyman limit ( $\alpha_{UV} = -1.5$ ,  $\alpha_X = -0.7$ );

**Table C21:** Simulations for  $v \geq 0$  of the region N0 of NGC 7212. For each bin there are the observed quantities and the results of the models. The first nine rows show the comparison between the observed and the synthetic spectra, the remaining rows show the input parameters of each model.

|                                             | bin 0 |                      | bin 1 |                      | bin 2 |       | bin 3 |       | bin 4 |       | bin 5 |       | bin 6 |      | bin 7 |       |
|---------------------------------------------|-------|----------------------|-------|----------------------|-------|-------|-------|-------|-------|-------|-------|-------|-------|------|-------|-------|
| line                                        | obs.  | mod.                 | obs.  | mod.                 | obs.  | mod.  | obs.  | mod.  | obs.  | mod.  | obs.  | mod.  | obs.  | mod. | obs.  | mod.  |
| [O II] $\lambda$ 3727+                      | 3.85  | 3.82                 | 3.9   | 4.18                 | 5.0   | 5.0   | 8.93  | 8.6   | 5.26  | 5.4   | 2.98  | 3.27  | 6.    | 5.9  | 8.1   | 8.3   |
| [Ne III] $\lambda$ 3869+                    | 2.0   | 1.9                  | 1.85  | 1.84                 | 2.05  | 2.09  | 3.6   | 3.22  | 2.79  | 2.33  | 3.1   | 2.2   | 2.6   | 2.5  | 0.4   | 1.3   |
| He II $\lambda$ 4686                        | 0.21  | 0.36                 | 0.2   | 0.3                  | 0.17  | 0.4   | 0.25  | 0.4   | 0.14  | 0.28  | 0.19  | 0.2   | 0.0   | 0.27 | 0.0   | 0.3   |
| [O III] $\lambda$ 5007+                     | 13.2  | 13.78                | 12.6  | 12.5                 | 12.43 | 12.58 | 13.44 | 13.3  | 9.89  | 10.0  | 7.98  | 7.99  | 8.59  | 8.5  | 9.2   | 9.2   |
| [O I] $\lambda$ 6300+,[S II] $\lambda$ 6310 | 0.56  | 0.22                 | 0.6   | 0.3                  | 0.61  | 0.60  | 0.56  | 0.51  | 0.5   | 0.5   | 0.54  | 0.7   | 0.71  | 0.9  | 0.59  | 0.6   |
| H $\alpha$                                  | 2.86  | 3.2                  | 2.86  | 3.2                  | 2.86  | 2.9   | 2.86  | 3.02  | 2.86  | 2.98  | 2.86  | 3.13  | 2.86  | 3.   | 2.86  | 3.    |
| [N II] $\lambda$ 6584                       | 2.0   | 2.15                 | 2.05  | 1.7                  | 1.95  | 2.4   | 1.88  | 1.6   | 1.88  | 1.7   | 1.62  | 1.4   | 1.78  | 2.   | 2.25  | 2.4   |
| [S II] $\lambda$ 6716                       | 1.0   | 0.9                  | 0.91  | 0.87                 | 0.73  | 1.0   | 0.73  | 0.78  | 1.07  | 0.85  | 1.04  | 0.6   | 0.4   | 0.68 | 0.52  | 0.7   |
| [S II] $\lambda$ 6731                       | 0.95  | 1.0                  | 0.83  | 1.1                  | 0.8   | 1.5   | 0.81  | 1.0   | 0.93  | 1.2   | 0.67  | 0.74  | 0.83  | 0.89 | 0.98  | 0.6   |
| FWHM(km s <sup>-1</sup> )                   | 0.0   | —                    | 100   | —                    | 200   | —     | 300   | —     | 400   | —     | 500   | —     | 600   | —    | 700   | —     |
| V <sub>s</sub> (km s <sup>-1</sup> )        | —     | 53                   | —     | 100                  | —     | 200   | —     | 300   | —     | 400   | —     | 500   | —     | 600  | —     | 700   |
| n <sub>0</sub> (cm <sup>-3</sup> )          | —     | 250                  | —     | 180                  | —     | 120   | —     | 100   | —     | 100   | —     | 100   | —     | 60   | —     | 20    |
| D(10 <sup>18</sup> cm)                      | —     | 0.0013               | —     | 0.0027               | —     | 0.17  | —     | 0.28  | —     | 0.5   | —     | 0.5   | —     | 0.25 | —     | 1.1   |
| F (units <sup>1</sup> )                     | —     | 0.21                 | —     | 0.26                 | —     | 2.6   | —     | 2.7   | —     | 1.7   | —     | 3.0   | —     | 0.9  | —     | 0.2   |
| O/H (10 <sup>4</sup> )                      | —     | 6.6                  | —     | 6.6                  | —     | 6.6   | —     | 6.6   | —     | 6.6   | —     | 6.6   | —     | 6.6  | —     | 6.6   |
| N/H (10 <sup>4</sup> )                      | —     | 1.2                  | —     | 1.2                  | —     | 0.7   | —     | 0.3   | —     | 0.4   | —     | 0.5   | —     | 0.5  | —     | 0.5   |
| Ne/H(10 <sup>4</sup> )                      | —     | 1.5                  | —     | 1.5                  | —     | 1.5   | —     | 1.5   | —     | 1.5   | —     | 1.9   | —     | 1.7  | —     | 0.8   |
| S/H (10 <sup>4</sup> )                      | —     | 0.6                  | —     | 0.9                  | —     | 0.2   | —     | 0.08  | —     | 0.08  | —     | 0.08  | —     | 0.08 | —     | 0.05  |
| H $\beta$ (erg)                             | —     | $1.7 \times 10^{-4}$ | —     | $3.6 \times 10^{-4}$ | —     | 0.048 | —     | 0.047 | —     | 0.033 | —     | 0.077 | —     | 0.02 | —     | 0.004 |

<sup>1</sup> in 10<sup>10</sup> phot cm<sup>-2</sup>s<sup>-1</sup>eV<sup>-1</sup> at the Lyman limit ( $\alpha_{UV} = -1.5$ ,  $\alpha_X = -0.7$ );



**Table C22:** Simulations for  $V < 0$  of the region N0 of NGC 7212. For each bin there are the observed quantities and the results of the models. The first nine rows show the comparison between the observed and the synthetic spectra, the remaining rows show the input parameters of each model.

| line                                        | bin -1 |          | bin -2 |      | bin -3 |       | bin -4 |       | bin -5 |       | bin -6 |      | bin -7 |      |
|---------------------------------------------|--------|----------|--------|------|--------|-------|--------|-------|--------|-------|--------|------|--------|------|
|                                             | obs.   | mod.     | obs.   | mod. | obs.   | mod.  | obs.   | mod.  | obs.   | mod.  | obs.   | mod. | obs.   | mod. |
| [O II] $\lambda$ 3727+                      | 4.04   | 4.4      | 3.78   | 3.8  | 4.5    | 4.1   | 4.58   | 4.9   | 3.5    | 3.57  | 9.1    | 9.3  | 3.65   | 30   |
| [Ne III] $\lambda$ 3869+                    | 1.94   | 1.95     | 1.5    | 2.   | 1.78   | 1.9   | 2.16   | 2.    | 1.7    | 1.89  | 7.5    | 3.1  | 6.95   | 1.8  |
| He II $\lambda$ 4686                        | 0.25   | 0.3      | 0.2    | 0.39 | 0.18   | 0.39  | 0.3    | 0.4   | 0.57   | 0.32  | 0.0    | 0.7  | 0.0    | 0.25 |
| [O III] $\lambda$ 5007+                     | 13.7   | 13.3     | 14.    | 14.2 | 14.7   | 14.7  | 14.98  | 15.   | 13.    | 12.83 | 17.4   | 17.  | 9.5    | 9.4  |
| [O I] $\lambda$ 6300+,[S II] $\lambda$ 6310 | 0.47   | 0.32     | 0.47   | 0.32 | 0.43   | 0.35  | 0.08   | 0.2   | 0.56   | 0.67  | 0.35   | 0.6  | 0.57   | 0.5  |
| H $\alpha$                                  | 2.86   | 3.16     | 2.86   | 2.89 | 2.86   | 2.9   | 2.86   | 2.9   | 2.86   | 2.93  | 2.86   | 3.1  | 2.86   | 3.   |
| [N II] $\lambda$ 6584                       | 1.99   | 1.8      | 1.9    | 2.   | 1.57   | 1.5   | 0.99   | 1.2   | 0.42   | 0.6   | 0.1    | 2.   | 0.013  | 0.6  |
| [S II] $\lambda$ 6716                       | 0.95   | 0.91     | 0.88   | 0.74 | 0.74   | 0.73  | 0.74   | 0.62  | 0.73   | 0.5   | 0.48   | 0.8  | 0.5    | 0.57 |
| [S II] $\lambda$ 6731                       | 0.92   | 1.2      | 0.83   | 1.2  | 0.77   | 1.26  | 0.55   | 1.0   | 1.0    | 0.93  | 0.86   | 0.8  | 0.12   | 0.9  |
| FWHM(km s $^{-1}$ )                         | -100   | —        | -200   | —    | -300   | —     | -400   | —     | -500   | —     | -600   | —    | -700   | —    |
| $V_s$ (km s $^{-1}$ )                       | —      | 100      | —      | 200  | —      | 300   | —      | 400   | —      | 500   | —      | 600  | —      | 700  |
| $n_0$ (cm $^{-3}$ )                         | —      | 180      | —      | 220  | —      | 160   | —      | 120   | —      | 150   | —      | 30   | —      | 64   |
| D(10 $^{18}$ cm)                            | —      | 0.0013   | —      | 0.04 | —      | 0.043 | —      | 0.052 | —      | 0.05  | —      | 1.7  | —      | 1.   |
| F (units $^1$ )                             | —      | 0.26     | —      | 4.5  | —      | 4.7   | —      | 3.6   | —      | 6.8   | —      | 3.0  | —      | 2.7  |
| O/H (10 $^4$ )                              | —      | 6.6      | —      | 6.6  | —      | 6.6   | —      | 6.6   | —      | 6.6   | —      | 6.6  | —      | 6.6  |
| N/H (10 $^4$ )                              | —      | 1.2      | —      | 0.7  | —      | 0.8   | —      | 0.6   | —      | 0.6   | —      | 0.6  | —      | 0.6  |
| Ne/H(10 $^4$ )                              | —      | 1.5      | —      | 1.5  | —      | 1.3   | —      | 1.3   | —      | 1.3   | —      | 1.3  | —      | 1.3  |
| S/H (10 $^4$ )                              | —      | 0.3      | —      | 0.2  | —      | 0.2   | —      | 0.15  | —      | 0.15  | —      | 0.15 | —      | 0.1  |
| H $\beta$ (erg)                             | —      | $3.4e-4$ | —      | 0.08 | —      | 0.07  | —      | 0.06  | —      | 0.13  | —      | 0.03 | —      | 0.06 |

$^1$  in  $10^{10}$  phot cm $^{-2}$ s $^{-1}$ eV $^{-1}$  at the Lyman limit ( $\alpha_{UV} = -1.5$ ,  $\alpha_X = -0.7$ );

**Table C23:** Simulations for  $V \geq 0$  of the region CN of NGC 7212, part 1. For each bin there are the observed quantities and the results of the models. The first nine rows show the comparison between the observed and the synthetic spectra, the remaining rows show the input parameters of each model.

|                                            | bin 0 |      | bin 1 |      | bin 2 |      | bin 3 |      | bin 4 |      | bin 5 |      |
|--------------------------------------------|-------|------|-------|------|-------|------|-------|------|-------|------|-------|------|
| line                                       | obs.  | mod. | obs.  | mod. | obs.  | mod. | obs.  | mod. | obs.  | mod. | obs.  | mod. |
| [O II] $\lambda$ 3727+                     | 2.82  | 2.65 | 2.93  | 3.01 | 3.04  | 3.17 | 3.18  | 3.05 | 3.61  | 3.56 | 3.39  | 3.7  |
| [Ne III] $\lambda$ 3869+                   | 1.96  | 1.94 | 2.0   | 2.1  | 2.09  | 2.08 | 2.22  | 2.3  | 2.07  | 2.74 | 2.54  | 2.4  |
| He II $\lambda$ 4686                       | 0.24  | 0.56 | 0.24  | 0.4  | 0.24  | 0.4  | 0.23  | 0.49 | 0.25  | 0.52 | 0.24  | 0.5  |
| [O III] $\lambda$ 5007+                    | 14.8  | 14.9 | 15.6  | 15.1 | 15.34 | 15.0 | 14.9  | 14.9 | 14.65 | 14.5 | 13.87 | 13.4 |
| [O I] $\lambda$ 6300,[S II] $\lambda$ 6310 | 0.61  | 0.75 | 0.62  | 0.74 | 0.61  | 0.64 | 0.6   | 1.0  | 0.60  | 0.8  | 0.72  | 0.85 |
| H $\alpha$                                 | 2.86  | 2.92 | 2.86  | 3.04 | 2.86  | 3.03 | 2.86  | 3.2  | 2.86  | 3.24 | 2.86  | 3.33 |
| [N II] $\lambda$ 6584                      | 1.99  | 2.12 | 1.94  | 1.98 | 1.91  | 2.0  | 1.88  | 2.14 | 1.79  | 2.3  | 1.79  | 2.28 |
| [S II] $\lambda$ 6716                      | 0.72  | 0.68 | 0.64  | 0.67 | 0.61  | 0.5  | 0.55  | 0.44 | 0.41  | 0.37 | 0.49  | 0.34 |
| [S II] $\lambda$ 6731                      | 0.85  | 0.78 | 0.78  | 1.0  | 0.72  | 0.81 | 0.69  | 0.76 | 0.61  | 0.66 | 0.64  | 1.61 |
| FWHM(km s $^{-1}$ )                        | 0.0   | —    | 100   | —    | 200   | —    | 300   | —    | 400   | —    | 500   | —    |
| $V_s$ (km s $^{-1}$ )                      | —     | 60   | —     | 90   | —     | 200  | —     | 300  | —     | 400  | —     | 510  |
| $n_0$ (cm $^{-3}$ )                        | —     | 230  | —     | 800  | —     | 450  | —     | 350  | —     | 240  | —     | 190  |
| D(10 $^{18}$ cm)                           | —     | 1.0  | —     | 0.7  | —     | 1.5  | —     | 0.2  | —     | 0.16 | —     | 0.14 |
| F (units $^1$ )                            | —     | 0.97 | —     | 15.  | —     | 14.  | —     | 30.  | —     | 26.  | —     | 25.  |
| O/H (10 $^4$ )                             | —     | 5.8  | —     | 6.5  | —     | 6.5  | —     | 6.6  | —     | 6.6  | —     | 6.6  |
| N/H (10 $^4$ )                             | —     | 0.8  | —     | 0.5  | —     | 0.5  | —     | 0.5  | —     | 0.5  | —     | 0.5  |
| Ne/H(10 $^4$ )                             | —     | 1.2  | —     | 1.0  | —     | 1.0  | —     | 1.0  | —     | 1.2  | —     | 1.1  |
| S/H (10 $^4$ )                             | —     | 0.04 | —     | 0.05 | —     | 0.05 | —     | 0.06 | —     | 0.06 | —     | 0.07 |
| H $\beta$ (erg)                            | —     | 0.06 | —     | 0.22 | —     | 0.21 | —     | 0.37 | —     | 0.32 | —     | 0.33 |

$^1$  in  $10^{10}$  phot cm $^{-2}$ s $^{-1}$ eV $^{-1}$  at the Lyman limit ( $\alpha_{UV} = -1.5$ ,  $\alpha_X = -0.7$ );

**Table C24:** Simulations for  $V \geq 0$  of the region CN of NGC 7212, part 2. For each bin there are the observed quantities and the results of the models. The first nine rows show the comparison between the observed and the synthetic spectra, the remaining rows show the input parameters of each model.

| line                                       | bin 6 |      | bin 7 |      | bin 8 |       | bin 9 |      |
|--------------------------------------------|-------|------|-------|------|-------|-------|-------|------|
|                                            | obs.  | mod. | obs.  | mod. | obs.  | mod.  | obs.  | mod. |
| [O II] $\lambda$ 3727+                     | 3.73  | 4.0  | 3.11  | 3.3  | 3.21  | 3.    | 2.12  | 2.6  |
| [Ne III] $\lambda$ 3869+                   | 2.61  | 0.94 | 2.0   | 2.17 | 2.1   | 1.8   | 1.26  | 1.3  |
| He II $\lambda$ 4686                       | 0.18  | 0.4  | 0.26  | 0.4  | 0.29  | 0.37  | 0.18  | 0.26 |
| [O III] $\lambda$ 5007+                    | 14.1  | 13.2 | 12.1  | 11.8 | 11.2  | 11.86 | 9.2   | 9.2  |
| [O I] $\lambda$ 6300,[S II] $\lambda$ 6310 | 0.97  | 1.0  | 0.99  | 0.77 | 0.83  | 0.72  | 0.73  | 0.7  |
| H $\alpha$                                 | 2.86  | 3.1  | 2.86  | 3.04 | 2.86  | 2.97  | 2.86  | 2.99 |
| [N II] $\lambda$ 6584                      | 1.96  | 2.2  | 2.07  | 1.93 | 2.2   | 1.65  | 2.06  | 1.8  |
| [S II] $\lambda$ 6716                      | 0.15  | 0.24 | 0.74  | 0.52 | 0.18  | 0.38  | 0.44  | 0.4  |
| [S II] $\lambda$ 6731                      | 0.63  | 0.45 | 0.69  | 1.0  | 0.65  | 0.76  | 0.6   | 0.67 |
| FWHM(km s $^{-1}$ )                        | 600   | —    | 700   | —    | 800   | —     | 900   | —    |
| $V_s$ (km s $^{-1}$ )                      | —     | 580  | —     | 700  | —     | 800   | —     | 900  |
| $n_0$ (cm $^{-3}$ )                        | —     | 190  | —     | 170  | —     | 150   | —     | 92.  |
| D(10 $^{18}$ cm)                           | —     | 0.08 | —     | 0.07 | —     | 0.06  | —     | 0.1  |
| F (units $^1$ )                            | —     | 22.  | —     | 22.  | —     | 21.   | —     | 8.   |
| O/H (10 $^4$ )                             | —     | 6.6  | —     | 6.6  | —     | 6.6   | —     | 6.5  |
| N/H (10 $^4$ )                             | —     | 0.6  | —     | 0.5  | —     | 0.5   | —     | 1.   |
| Ne/H(10 $^4$ )                             | —     | 1.3  | —     | 1.3  | —     | 1.3   | —     | 1.2  |
| S/H (10 $^4$ )                             | —     | 0.07 | —     | 0.2  | —     | 0.2   | —     | 0.15 |
| H $\beta$ (erg)                            | —     | 0.35 | —     | 0.4  | —     | 0.42  | —     | 0.2  |

$^1$  in 10 $^{10}$  phot cm $^{-2}$ s $^{-1}$ eV $^{-1}$  at the Lyman limit ( $\alpha_{UV} = -1.5$ ,  $\alpha_X = -0.7$ );

**Table C25:** Simulations for  $V < 0$  of the region CN of NGC 7212. For each bin there are the observed quantities and the results of the models. The first nine rows show the comparison between the observed and the synthetic spectra, the remaining rows show the input parameters of each model.

| line                                       | bin -1 |      | bin -2 |      | bin 3 |       | bin -4 |      | bin -5 |       | bin -6 |      | bin -7 |      | bin -8 |      |
|--------------------------------------------|--------|------|--------|------|-------|-------|--------|------|--------|-------|--------|------|--------|------|--------|------|
|                                            | obs.   | mod. | obs.   | mod. | obs.  | mod.  | obs.   | mod. | obs.   | mod.  | obs.   | mod. | obs.   | mod. | obs.   | mod. |
| [O II] $\lambda$ 3727+                     | 3.05   | 3.   | 2.75   | 2.78 | 2.74  | 2.7   | 3.     | 3.17 | 2.77   | 2.87  | 3.97   | 4.0  | 7.5    | 7.4  | 15.2   | 14.  |
| [Ne III] $\lambda$ 3869+                   | 2.0    | 2.1  | 1.76   | 2.   | 1.72  | 2.83  | 1.77   | 1.5  | 1.66   | 1.67  | 2.8    | 2.6  | 2.9    | 2.74 | 3.96   | 3.0  |
| He II $\lambda$ 4686                       | 0.23   | 0.43 | 0.21   | 0.38 | 0.23  | 0.47  | 0.2    | 0.37 | 0.12   | 0.3   | 0.18   | 0.46 | 0.11   | 0.6  | 0.0    | 0.79 |
| [O III] $\lambda$ 5007+                    | 15.    | 15.1 | 14.5   | 14.3 | 14.3  | 14.5  | 14.2   | 14.2 | 14.4   | 14.36 | 14.    | 14.3 | 15.2   | 14.8 | 21.56  | 15.2 |
| [O I] $\lambda$ 6300,[S II] $\lambda$ 6310 | 0.62   | 0.8  | 0.56   | 0.7  | 0.5   | 0.9   | 0.52   | 0.5  | 0.53   | 0.4   | 0.41   | 0.5  | 0.35   | 0.4  | 0.42   | 0.3  |
| H $\alpha$                                 | 2.86   | 3.   | 2.86   | 3.   | 2.86  | 3.2   | 2.86   | 2.9  | 2.86   | 2.93  | 2.86   | 3.   | 2.86   | 2.97 | 2.86   | 4.2  |
| [N II] $\lambda$ 6584                      | 1.93   | 1.98 | 1.85   | 2.0  | 1.78  | 1.7   | 1.83   | 2.   | 1.4    | 1.75  | 1.26   | 1.77 | 1.36   | 1.5  | 1.31   | 1.5  |
| [S II] $\lambda$ 6716                      | 0.72   | 0.67 | 0.71   | 0.61 | 0.63  | 0.55  | 0.62   | 0.5  | 0.67   | 0.44  | 0.58   | 0.35 | 0.43   | 0.41 | 0.18   | 0.48 |
| [S II] $\lambda$ 6731                      | 0.85   | 1.0  | 0.85   | 1.   | 0.876 | 0.96  | 0.82   | 1.0  | 0.69   | 0.89  | 1.27   | 1.13 | 0.63   | 0.74 | 1.7    | 0.47 |
| FWHM(km s $^{-1}$ )                        | -100   | —    | -200   | —    | -300  | —     | -400   | —    | -500   | —     | -600   | —    | -700   | —    | -800   | —    |
| V <sub>s</sub> (km s $^{-1}$ )             | —      | 90   | —      | 200  | —     | 300   | —      | 400  | —      | 500   | —      | 600  | —      | 700  | —      | 870  |
| n <sub>0</sub> (cm $^{-3}$ )               | —      | 800  | —      | 530  | —     | 400   | —      | 300  | —      | 280   | —      | 180  | —      | 95   | —      | 20   |
| D(10 $^{18}$ cm)                           | —      | 0.7  | —      | 1.4  | —     | 0.17  | —      | 0.03 | —      | 0.018 | —      | 0.07 | —      | 0.13 | —      | 8.3  |
| F (units $^1$ )                            | —      | 15.  | —      | 17.  | —     | 35.   | —      | 19.  | —      | 12.5  | —      | 23.  | —      | 17.  | —      | 26.6 |
| O/H (10 $^4$ )                             | —      | 6.5  | —      | 6.5  | —     | 6.5   | —      | 6.5  | —      | 6.6   | —      | 6.6  | —      | 6.6  | —      | 6.7  |
| N/H (10 $^4$ )                             | —      | 0.5  | —      | 0.5  | —     | 0.5   | —      | 0.5  | —      | 0.5   | —      | 0.4  | —      | 0.3  | —      | 0.3  |
| Ne/H(10 $^4$ )                             | —      | 1.0  | —      | 1.0  | —     | 0.8   | —      | 0.8  | —      | 1.    | —      | 1.3  | —      | 1.4  | —      | 1.3  |
| S/H (10 $^4$ )                             | —      | 0.05 | —      | 0.07 | —     | 0.086 | —      | 0.2  | —      | 0.2   | —      | 0.2  | —      | 0.2  | —      | 0.4  |
| H $\beta$ (erg)                            | —      | 0.2  | —      | 0.26 | —     | 0.45  | —      | 0.36 | —      | 0.23  | —      | 0.35 | —      | 0.21 | —      | 0.23 |

<sup>1</sup> in 10 $^{10}$  phot cm $^{-2}$ s $^{-1}$ eV $^{-1}$  at the Lyman limit ( $\alpha_{UV} = -1.5$ ,  $\alpha_X = -0.7$ );

**Table C26:** Simulations for  $V \geq 0$  of the region CS of NGC 7212, part 1. For each bin there are the observed quantities and the results of the models. The first nine rows show the comparison between the observed and the synthetic spectra, the remaining rows show the input parameters of each model.

|                          | bin 0 |       | bin 1 |      | bin 2 |      | bin 3 |      | bin 4 |      | bin 5 |      | bin 6 |       |
|--------------------------|-------|-------|-------|------|-------|------|-------|------|-------|------|-------|------|-------|-------|
| line                     | obs.  | mod.  | obs.  | mod. | obs.  | mod. | obs.  | mod. | obs.  | mod. | obs.  | mod. | obs.  | mod.  |
| [O II] $\lambda$ 3727+   | 3.34  | 3.3   | 2.5   | 3.1  | 2.24  | 2.3  | 2.26  | 2.46 | 2.34  | 2.67 | 2.58  | 2.5  | 2.5   | 2.7   |
| [Ne III] $\lambda$ 3869+ | 1.95  | 2.0   | 1.81  | 1.75 | 1.85  | 1.9  | 1.9   | 1.9  | 2.08  | 1.9  | 2.44  | 1.7  | 2.56  | 2.3   |
| He II $\lambda$ 4686     | 0.23  | 0.59  | 0.23  | 0.4  | 0.23  | 0.5  | 0.22  | 0.49 | 0.23  | 0.5  | 0.23  | 0.5  | 0.17  | 0.24  |
| [O III] $\lambda$ 5007+  | 16.2  | 16.1  | 15.85 | 15.7 | 16.6  | 16.8 | 16.25 | 16.0 | 15.5  | 15.3 | 14.3  | 14.3 | 13.8  | 14.   |
| [O I] $\lambda$ 6300+    | 0.2   | 0.12  | 0.2   | 0.1  | 0.27  | 0.11 | 0.56  | 0.54 | 0.53  | 0.54 | 1.54  | 0.2  | 0.64  | 0.1   |
| H $\alpha$               | 2.86  | 2.95  | 2.86  | 2.97 | 2.86  | 3.0  | 2.86  | 3.2  | 2.86  | 3.2  | 2.86  | 3.2  | 2.86  | 2.87  |
| [N II] $\lambda$ 6584    | 1.8   | 1.86  | 1.85  | 1.77 | 1.8   | 1.7  | 1.77  | 1.82 | 1.68  | 1.86 | 1.52  | 1.7  | 1.4   | 1.67  |
| [S II] $\lambda$ 6716    | 0.67  | 0.63  | 0.6   | 0.42 | 0.53  | 0.3  | 0.5   | 0.3  | 0.43  | 0.3  | 0.32  | 0.22 | 0.38  | 0.34  |
| [S II] $\lambda$ 6731    | 0.72  | 0.71  | 0.73  | 0.77 | 0.66  | 0.6  | 0.6   | 0.6  | 0.55  | 0.6  | 0.46  | 0.46 | 0.44  | 0.78  |
| FWHM(km s $^{-1}$ )      | 0.0   | —     | 100   | —    | 200   | —    | 300   | —    | 400   | —    | 500   | —    | 600   | —     |
| $V_s$ (km s $^{-1}$ )    | —     | 60    | —     | 100  | —     | 200  | —     | 300  | —     | 400  | —     | 530  | —     | 600   |
| $n_0$ (cm $^{-3}$ )      | —     | 220   | —     | 900  | —     | 700  | —     | 500  | —     | 400  | —     | 360  | —     | 300   |
| D(10 $^{18}$ cm)         | —     | 1.0   | —     | 0.05 | —     | 0.05 | —     | 0.05 | —     | 0.05 | —     | 0.04 | —     | 0.008 |
| F (units $^1$ )          | —     | 1.2   | —     | 15.  | —     | 42.  | —     | 46.  | —     | 46.  | —     | 47.  | —     | 7.2   |
| O/H (10 $^4$ )           | —     | 6.6   | —     | 6.6  | —     | 6.6  | —     | 6.6  | —     | 6.6  | —     | 6.6  | —     | 6.6   |
| N/H (10 $^4$ )           | —     | 0.6   | —     | 0.4  | —     | 0.4  | —     | 0.4  | —     | 0.4  | —     | 0.4  | —     | 0.5   |
| Ne/H(10 $^4$ )           | —     | 1.2   | —     | 0.8  | —     | 0.8  | —     | 0.8  | —     | 0.8  | —     | 0.8  | —     | 1.4   |
| S/H (10 $^4$ )           | —     | 0.04  | —     | 0.07 | —     | 0.07 | —     | 0.08 | —     | 0.09 | —     | 0.09 | —     | 0.2   |
| H $\beta$ (erg)          | —     | 0.054 | —     | 0.22 | —     | 0.53 | —     | 0.59 | —     | 0.6  | —     | 0.73 | —     | 0.17  |

$^1$  in 10 $^{10}$  phot cm $^{-2}$ s $^{-1}$ eV $^{-1}$  at the Lyman limit ( $\alpha_{UV} = -1.5$ ,  $\alpha_X = -0.7$ );

**Table C27:** Simulations for  $V \geq 0$  of the region CS of NGC 7212, part 2. For each bin there are the observed quantities and the results of the models. The first nine rows show the comparison between the observed and the synthetic spectra, the remaining rows show the input parameters of each model.

| line                     | bin 7 |      | bin 8 |      | bin 9 |      |
|--------------------------|-------|------|-------|------|-------|------|
|                          | obs.  | mod. | obs.  | mod. | obs.  | mod. |
| [O II] $\lambda$ 3727+   | 3.77  | 3.3  | 3.54  | 3.9  | 3.69  | 3.0  |
| [Ne III] $\lambda$ 3869+ | 3.23  | 3.   | 3.18  | 2.4  | 2.23  | 2.2  |
| He II $\lambda$ 4686     | 0.23  | 0.33 | 0.19  | 0.3  | 0.22  | 0.26 |
| [O III] $\lambda$ 5007+  | 14.   | 15.  | 11.6  | 11.6 | 9.77  | 9.83 |
| [O I] $\lambda$ 6300+    | 0.73  | 0.1  | 0.73  | 0.4  | 0.62  | 0.76 |
| H $\alpha$               | 2.86  | 2.87 | 2.86  | 2.92 | 2.86  | 2.98 |
| [N II] $\lambda$ 6584    | 1.3   | 1.5  | 1.27  | 1.6  | 1.26  | 1.44 |
| [S II] $\lambda$ 6716    | 0.3   | 0.4  | 0.48  | 0.45 | 0.38  | 0.3  |
| [S II] $\lambda$ 6731    | 0.37  | 0.8  | 0.37  | 0.8  | 0.31  | 0.49 |
| FWHM(km s $^{-1}$ )      | 700   | —    | 800   | —    | 900   | —    |
| V $_s$ (km s $^{-1}$ )   | —     | 690  | —     | 800  | —     | 900  |
| n $_0$ (cm $^{-3}$ )     | —     | 180  | —     | 105  | —     | 92   |
| D(10 $^{18}$ cm)         | —     | 0.02 | —     | 0.06 | —     | 0.1  |
| F (units $^1$ )          | —     | 8.5  | —     | 9.1  | —     | 7.9  |
| O/H (10 $^4$ )           | —     | 6.7  | —     | 6.6  | —     | 6.7  |
| Ne/H(10 $^4$ )           | —     | 0.5  | —     | 0.5  | —     | 0.5  |
| Ne/H(10 $^4$ )           | —     | 1.9  | —     | 1.9  | —     | 1.9  |
| S/H (10 $^4$ )           | —     | 0.2  | —     | 0.2  | —     | 0.1  |
| H $\beta$ (erg)          | —     | 0.2  | —     | 0.19 | —     | 0.19 |

$^1$  in  $10^{10}$  phot cm $^{-2}$ s $^{-1}$ eV $^{-1}$  at the Lyman limit ( $\alpha_{UV} = -1.5$ ,  $\alpha_X = -0.7$ );

**Table C28:** Simulations for  $V < 0$  of the region CS of NGC 7212. For each bin there are the observed quantities and the results of the models. The first nine rows show the comparison between the observed and the synthetic spectra, the remaining rows show the input parameters of each model.

|                                            | bin -1 |      | bin -2 |       | bin -3 |       | bin -4 |        | bin -5 |        | bin -6 |       | bin -7 |      |
|--------------------------------------------|--------|------|--------|-------|--------|-------|--------|--------|--------|--------|--------|-------|--------|------|
| line                                       | obs.   | mod. | obs.   | mod.  | obs.   | mod.  | obs.   | mod.   | obs.   | mod.   | obs.   | mod.  | obs.   | mod. |
| [O II] $\lambda$ 3727+                     | 2.06   | 2.06 | 2.8    | 2.7   | 3.27   | 3.    | 3.07   | 3.22   | 3.     | 3.     | 6.58   | 6.4   | 5.93   | 5.7  |
| [Ne III] $\lambda$ 3869+                   | 1.64   | 1.63 | 1.36   | 1.45  | 1.8    | 1.7   | 1.62   | 1.77   | 2.22   | 2.1    | 1.34   | 1.68  | 1.52   | 1.5  |
| He II $\lambda$ 4686                       | 0.19   | 0.37 | 0.19   | 0.38  | 0.21   | 0.3   | 0.23   | 0.36   | 0.19   | 0.3    | 0.15   | 0.4   | 0.0    | 0.3  |
| [O III] $\lambda$ 5007+                    | 14.4   | 14.2 | 14.    | 14.5  | 13.4   | 13.2  | 14.25  | 14.47  | 13.4   | 13.1   | 12.93  | 13.2  | 11.33  | 11.8 |
| [O I] $\lambda$ 6300,[S II] $\lambda$ 6310 | 0.55   | 0.6  | 0.47   | 0.4   | 0.39   | 0.4   | 0.43   | 0.42   | 0.28   | 0.26   | 0.21   | 0.6   | 0.8    | 1.2  |
| H $\alpha$                                 | 2.86   | 2.96 | 2.86   | 2.98  | 2.86   | 2.9   | 2.86   | 2.9    | 2.86   | 2.9    | 2.86   | 3.13  | 2.86   | 2.95 |
| [N II] $\lambda$ 6584                      | 1.85   | 1.63 | 1.42   | 1.4   | 1.11   | 1.0   | 0.88   | 1.0    | 0.39   | 0.6    | 0.08   | 0.6   | 0.0    | 0.6  |
| [S II] $\lambda$ 6716                      | 0.83   | 0.6  | 0.66   | 0.5   | 0.5    | 0.4   | 0.57   | 0.4    | 0.54   | 0.4    | 0.4    | 0.8   | 0.44   | 0.5  |
| [S II] $\lambda$ 6731                      | 0.81   | 1.0  | 0.71   | 0.99  | 0.58   | 0.8   | 0.47   | 0.76   | 0.52   | 0.76   | 0.8    | 1.3   | 0.66   | 0.87 |
| FWHM(km s <sup>-1</sup> )                  | -100   | —    | -200   | —     | -300   | —     | -400   | —      | -500   | —      | -600   | —     | -700   | —    |
| V <sub>s</sub> (km s <sup>-1</sup> )       | —      | 120  | —      | 200   | —      | 300   | —      | 400    | —      | 500    | —      | 600   | —      | 700  |
| n <sub>0</sub> (cm <sup>-3</sup> )         | —      | 1200 | —      | 500   | —      | 350   | —      | 290    | —      | 270    | —      | 100   | —      | 100  |
| D(10 <sup>18</sup> cm)                     | —      | 0.02 | —      | 0.024 | —      | 0.024 | —      | 0.0247 | —      | 0.0245 | —      | 0.2   | —      | 0.54 |
| F (units <sup>1</sup> )                    | —      | 23.  | —      | 14.   | —      | 14.   | —      | 16.    | —      | 16.    | —      | 1.    | —      | 0.34 |
| O/H (10 <sup>4</sup> )                     | —      | 6.6  | —      | 6.6   | —      | 6.6   | —      | 6.6    | —      | 6.6    | —      | 6.6   | —      | 6.6  |
| N/H (10 <sup>4</sup> )                     | —      | 0.4  | —      | 0.4   | —      | 0.4   | —      | 0.4    | —      | 0.3    | —      | 0.2   | —      | 0.2  |
| Ne/H(10 <sup>4</sup> )                     | —      | 0.8  | —      | 0.8   | —      | 1.0   | —      | 1.0    | —      | 1.2    | —      | 0.8   | —      | 0.8  |
| S/H (10 <sup>4</sup> )                     | —      | 0.16 | —      | 0.16  | —      | 0.16  | —      | 0.16   | —      | 0.16   | —      | 0.15  | —      | 0.07 |
| H $\beta$ (erg)                            | —      | 0.37 | —      | 0.23  | —      | 0.3   | —      | 0.31   | —      | 0.33   | —      | 0.146 | —      | 0.02 |

<sup>1</sup> in 10<sup>10</sup> phot cm<sup>-2</sup>s<sup>-1</sup>eV<sup>-1</sup> at the Lyman limit ( $\alpha_{UV} = -1.5$ ,  $\alpha_X = -0.7$ );

**Table C29:** Simulations for  $V \geq 0$  of the region S0 of NGC 7212. For each bin there are the observed quantities and the results of the models. The first nine rows show the comparison between the observed and the synthetic spectra, the remaining rows show the input parameters of each model.

|                                             | bin 0 |       | bin 1 |      | bin 2 |      | bin 3 |      | bin 4 |       | bin 5 |       |
|---------------------------------------------|-------|-------|-------|------|-------|------|-------|------|-------|-------|-------|-------|
| line                                        | obs.  | mod.  | obs.  | mod. | obs.  | mod. | obs.  | mod. | obs.  | mod.  | obs.  | mod.  |
| [O II] $\lambda$ 3727+                      | 3.57  | 3.3   | 2.75  | 2.73 | 3.1   | 3.3  | 1.4   | 2.1  | 2.5   | 2.78  | 3.9   | 4.1   |
| [Ne III] $\lambda$ 3869+                    | 1.8   | 2.0   | 2.27  | 2.68 | 2.1   | 2.2  | 2.1   | 2.3  | 2.    | 2.2   | 2.2   | 2.38  |
| He II $\lambda$ 4686                        | 0.22  | 0.59  | 0.2   | 0.4  | 0.22  | 0.5  | 0.22  | 0.46 | 0.18  | 0.5   | 0.0   | 0.6   |
| [O III] $\lambda$ 5007+                     | 16.3  | 16.1  | 15.5  | 16.2 | 16.1  | 15.3 | 15.2  | 15.1 | 13.63 | 13.65 | 13.75 | 13.43 |
| [O I] $\lambda$ 6300+,[S II] $\lambda$ 6310 | 0.38  | 0.5   | 0.35  | 0.8  | 0.5   | 0.8  | 0.51  | 0.7  | 0.7   | 0.9   | 0.7   | 0.8   |
| H $\alpha$                                  | 2.86  | 2.95  | 2.86  | 3.   | 2.86  | 3.13 | 2.86  | 3.13 | 2.86  | 3.2   | 2.86  | 3.36  |
| [N II] $\lambda$ 6584                       | 1.7   | 1.86  | 1.72  | 1.7  | 1.78  | 1.65 | 1.71  | 1.6  | 1.67  | 1.84  | 1.67  | 2.1   |
| [S II] $\lambda$ 6716                       | 0.63  | 0.63  | 0.51  | 0.4  | 0.42  | 0.3  | 0.35  | 0.4  | 0.6   | 0.4   | 0.6   | 0.3   |
| [S II] $\lambda$ 6731                       | 0.58  | 0.71  | 0.64  | 0.5  | 0.67  | 0.5  | 0.59  | 0.8  | 0.6   | 0.7   | 0.6   | 0.54  |
| FWHM(km s $^{-1}$ )                         | 0.0   | —     | 100   | —    | 200   | —    | 300   | —    | 400   | —     | 500   | —     |
| V <sub>s</sub> (km s $^{-1}$ )              | —     | 60    | —     | 110  | —     | 200  | —     | 280  | —     | 400   | —     | 500   |
| n <sub>0</sub> (cm $^{-3}$ )                | —     | 220   | —     | 920  | —     | 420  | —     | 550  | —     | 350   | —     | 260   |
| D(10 $^{18}$ cm)                            | —     | 1.    | —     | 0.18 | —     | 0.12 | —     | 0.1  | —     | 0.1   | —     | 0.075 |
| F (units $^1$ )                             | —     | 1.2   | —     | 20.  | —     | 25.  | —     | 45.  | —     | 48.   | —     | 46.   |
| O/H (10 $^4$ )                              | —     | 6.6   | —     | 6.6  | —     | 6.6  | —     | 6.6  | —     | 6.6   | —     | 6.6   |
| N/H (10 $^4$ )                              | —     | 0.6   | —     | 0.4  | —     | 0.4  | —     | 0.4  | —     | 0.4   | —     | 0.4   |
| Ne/H(10 $^4$ )                              | —     | 1.2   | —     | 1.2  | —     | 1.0  | —     | 1.0  | —     | 1.0   | —     | 1.0   |
| S/H (10 $^4$ )                              | —     | 0.04  | —     | 0.04 | —     | 0.04 | —     | 0.08 | —     | 0.08  | —     | 0.09  |
| H $\beta$ (erg)                             | —     | 0.054 | —     | 0.28 | —     | 0.31 | —     | 0.6  | —     | 0.61  | —     | 0.58  |

$^1$  in  $10^{10}$  phot cm $^{-2}$ s $^{-1}$ eV $^{-1}$  at the Lyman limit ( $\alpha_{UV} = -1.5$ ,  $\alpha_X = -0.7$ );



**Table C30:** Simulations for  $V < 0$  of the region S0 of NGC 7212. For each bin there are the observed quantities and the results of the models. The first nine rows show the comparison between the observed and the synthetic spectra, the remaining rows show the input parameters of each model.

| line                                        | bin -1 |      | bin -2 |      | bin -3 |      | bin -4 |      | bin -5 |      |
|---------------------------------------------|--------|------|--------|------|--------|------|--------|------|--------|------|
|                                             | obs.   | mod. | obs.   | mod. | obs.   | mod. | obs.   | mod. | obs.   | mod. |
| [O II] $\lambda$ 3727+                      | 3.06   | 2.9  | 2.6    | 2.7  | 4.28   | 4.7  | 3.94   | 3.6  | 3.9    | 4.2  |
| [Ne III] $\lambda$ 3869+                    | 1.3    | 1.6  | 0.78   | 1.2  | 1.7    | 1.6  | 0.77   | 0.87 | 4.8    | 1.1  |
| He II $\lambda$ 4686                        | 0.16   | 0.3  | 0.09   | 0.2  | 0.18   | 0.3  | 0.16   | 0.3  | 0.03   | 0.4  |
| [O III] $\lambda$ 5007+                     | 12.1   | 12.4 | 7.66   | 7.53 | 11.5   | 11.4 | 12.26  | 12.5 | 17.63  | 17.  |
| [O I] $\lambda$ 6300+,[S II] $\lambda$ 6310 | 0.42   | 0.6  | 0.34   | 0.4  | 0.21   | 0.6  | 0.37   | 0.3  | 0.22   | 0.2  |
| H $\alpha$                                  | 2.86   | 2.97 | 2.86   | 3.   | 2.86   | 2.95 | 2.86   | 2.92 | 2.86   | 2.89 |
| [N II] $\lambda$ 6584                       | 1.85   | 1.5  | 1.75   | 1.6  | 1.85   | 1.6  | 2.1    | 2.1  | 0.92   | 0.75 |
| [S II] $\lambda$ 6716                       | 0.9    | 0.53 | 0.9    | 0.86 | 1.0    | 1.5  | 1.26   | 0.6  | 1.87   | 0.9  |
| [S II] $\lambda$ 6731                       | 0.72   | 0.88 | 0.7    | 1.5  | 0.86   | 2.2  | 1.44   | 1.2  | 2.39   | 1.8  |
| FWHM(km s $^{-1}$ )                         | -100   | —    | -200   | —    | -300   | —    | -400   | —    | -500   | —    |
| V <sub>s</sub> (km s $^{-1}$ )              | —      | 100  | —      | 200  | —      | 300  | —      | 400  | —      | 500  |
| n <sub>0</sub> (cm $^{-3}$ )                | —      | 900  | —      | 550  | —      | 200  | —      | 200  | —      | 170  |
| D(10 $^{18}$ cm)                            | —      | 0.2  | —      | 0.35 | —      | 0.25 | —      | 0.03 | —      | 0.03 |
| F (units $^1$ )                             | —      | 10.  | —      | 6.   | —      | 3.4  | —      | 6.   | —      | 10.  |
| O/H (10 $^4$ )                              | —      | 6.6  | —      | 6.6  | —      | 6.6  | —      | 6.6  | —      | 6.6  |
| N/H (10 $^4$ )                              | —      | 0.6  | —      | 0.6  | —      | 0.6  | —      | 0.6  | —      | 0.4  |
| Ne/H(10 $^4$ )                              | —      | 0.9  | —      | 0.9  | —      | 0.9  | —      | 0.6  | —      | 0.6  |
| S/H (10 $^4$ )                              | —      | 0.06 | —      | 0.15 | —      | 0.13 | —      | 0.18 | —      | 0.4  |
| H $\beta$ (erg)                             | —      | 0.18 | —      | 0.14 | —      | 0.06 | —      | 0.12 | —      | 0.14 |

$^1$  in  $10^{10}$  phot cm $^{-2}$ s $^{-1}$ eV $^{-1}$  at the Lyman limit ( $\alpha_{UV} = -1.5$ ,  $\alpha_X = -0.7$ );

**Table C31:** Simulations for  $V \geq 0$  of the region S1 of NGC 7212. For each bin there are the observed quantities and the results of the models. The first nine rows show the comparison between the observed and the synthetic spectra, the remaining rows show the input parameters of each model.

| line                                         | bin 0 |       | bin 1 |       | bin 2 |       | bin 3 |       | bin 4 |        | bin 5 |       |
|----------------------------------------------|-------|-------|-------|-------|-------|-------|-------|-------|-------|--------|-------|-------|
|                                              | obs.  | mod.  | obs.  | mod.  | obs.  | mod.  | obs.  | mod.  | obs.  | mod.   | obs.  | mod.  |
| [O II] $\lambda$ 3727+                       | 5.1   | 5.0   | 4.4   | 4.3   | 6.48  | 6.9   | 0.52  | 3.5*  | 1.9   | 2.     | 3.5   | 3.5   |
| [Ne III] $\lambda$ 3869+                     | 1.9   | 1.76  | 5.6   | 3.1   | 1.0   | 1.7*  | 0.0   | 1.47  | 0.    | 1.37   | 0.0   | 1.67  |
| He II $\lambda$ 4686                         | 0.30  | 0.8   | 0.67  | 0.9   | 0.26  | 0.8   | 0.0   | 0.4   | 0.0   | 0.35   | 0.0   | 0.5   |
| [O III] $\lambda$ 5007+                      | 17.25 | 17.7  | 20.5  | 22.3  | 19.1  | 20.   | 16.5  | 16.9  | 14.   | 13.7   | 16.0  | 15.83 |
| [O I] $\lambda$ 6300+,[S III] $\lambda$ 6312 | 0.42  | 0.32  | 0.57  | 0.2   | 0.99  | 0.95  | 1.04  | 0.7   | 1.5   | 0.5    | 2.7   | 1.0   |
| H $\alpha$                                   | 2.86  | 2.87  | 2.86  | 2.9   | 2.86  | 3.    | 2.86  | 2.9   | 2.0   | 2.9    | 2.89  | 2.97  |
| [N II] $\lambda$ 6584                        | 1.7   | 1.44  | 1.82  | 1.74  | 1.98  | 2.12  | 1.6   | 1.73  | 1.5   | 1.6    | 2.89  | 2.14  |
| [S II] $\lambda$ 6716                        | 0.71  | 0.67  | 0.44  | 0.35  | 0.7   | 0.85  | 0.67  | 0.53  | 0.0   | 0.25   | —     | 0.3   |
| [S II] $\lambda$ 6731                        | 0.55  | 0.62  | 0.66  | 0.43  | 0.7   | 1.1   | 0.7   | 1.0   | 0.54  | 0.56   | 0.0   | 0.7   |
| FWHM(km s <sup>-1</sup> )                    | 0.0   | —     | 100   | —     | 200   | —     | 300   | —     | 400   | —      | 500   | —     |
| V <sub>s</sub> (km s <sup>-1</sup> )         | —     | 60    | —     | 100   | —     | 190   | —     | 300   | —     | 400    | —     | 500   |
| n <sub>0</sub> (cm <sup>-3</sup> )           | —     | 110   | —     | 150   | —     | 120   | —     | 300   | —     | 500    | —     | 280   |
| D(10 <sup>18</sup> cm)                       | —     | 0.7   | —     | 0.16  | —     | 0.16  | —     | 0.018 | —     | 0.0064 | —     | 0.035 |
| F (units <sup>1</sup> )                      | —     | 1.3   | —     | 4.3   | —     | 5.7   | —     | 10.   | —     | 20.    | —     | 40.   |
| O/H (10 <sup>4</sup> )                       | —     | 6.6   | —     | 6.6   | —     | 6.6   | —     | 6.6   | —     | 6.6    | —     | 6.6   |
| N/H (10 <sup>4</sup> )                       | —     | 0.6   | —     | 1.0   | —     | 0.6   | —     | 0.5   | —     | 0.5    | —     | 0.5   |
| Ne/H(10 <sup>4</sup> )                       | —     | 1.2   | —     | 1.8   | —     | 0.8   | —     | 0.8   | —     | 0.8    | —     | 0.8   |
| S/H (10 <sup>4</sup> )                       | —     | 0.35  | —     | 0.4   | —     | 0.35  | —     | 0.2   | —     | 0.2    | —     | 0.2   |
| H $\beta$ (erg)                              | —     | 0.012 | —     | 0.024 | —     | 0.039 | —     | 0.15  | —     | 0.4    | —     | 0.6   |

<sup>1</sup> in 10<sup>10</sup> phot cm<sup>-2</sup>s<sup>-1</sup>eV<sup>-1</sup> at the Lyman limit ( $\alpha_{UV} = -1.5$ ,  $\alpha_X = -0.7$ );

**Table C32:** Simulations for  $V < 0$  of the region S1 of NGC 7212. For each bin there are the observed quantities and the results of the models. The first nine rows show the comparison between the observed and the synthetic spectra, the remaining rows show the input parameters of each model.

| line                                        | bin -1 |       | bin -2 |      | bin -3 |       | bin -4 |       | bin -5 |       |
|---------------------------------------------|--------|-------|--------|------|--------|-------|--------|-------|--------|-------|
|                                             | obs.   | mod.  | obs.   | mod. | obs.   | mod.  | obs.   | mod.  | obs.   | mod.  |
| [O II] $\lambda$ 3727+                      | 3.16   | 3.5   | 2.63   | 2.8  | 5.8    | 5.7   | 6.65   | 6.6   | 3.17   | 3.5   |
| [Ne III] $\lambda$ 3869+                    | 1.     | 1.5   | 0.73   | 1.1  | 1.45   | 1.62  | 0.75   | 1.7   | 0.0    | 2.7   |
| He II $\lambda$ 4686                        | 0.07   | 0.39  | 0.08   | 0.2  | 0.0    | 0.3   | 0.0    | 0.4   | 0.0    | 0.3   |
| [O III] $\lambda$ 5007+                     | 10.73  | 10.22 | 7.3    | 7.5  | 11.6   | 11.66 | 15.    | 14.83 | 30.73  | 25.   |
| [O I] $\lambda$ 6300+,[S II] $\lambda$ 6310 | 0.43   | 0.5   | 0.4    | 0.4  | 0.9    | 1.0   | 1.9    | 1.7   | 0.81   | 0.1   |
| H $\alpha$                                  | 2.86   | 2.97  | 2.86   | 3.   | 2.86   | 2.97  | 2.53   | 3.2   | 2.86   | 3.8   |
| [N II] $\lambda$ 6584                       | 1.64   | 1.6   | 1.81   | 2.1  | 2.35   | 2.4   | 4.7    | 2.34  | 8.32   | 1.8   |
| [S II] $\lambda$ 6716                       | 0.76   | 1.    | 0.91   | 0.6  | 1.34   | 1.62  | 1.73   | 1.56  | 3.12   | 0.3   |
| [S II] $\lambda$ 6731                       | 0.59   | 1.6   | 0.69   | 1.   | 1.25   | 2.1   | 2.05   | 1.9   | 3.05   | 0.5   |
| FWHM(km s $^{-1}$ )                         | -100   | —     | -200   | —    | -300   | —     | -400   | —     | -500   | —     |
| V <sub>s</sub> (km s $^{-1}$ )              | —      | 110   | —      | 200  | —      | 300   | —      | 400   | —      | 500   |
| n <sub>0</sub> (cm $^{-3}$ )                | —      | 580   | —      | 580  | —      | 140   | —      | 70    | —      | 100   |
| D(10 $^{18}$ cm)                            | —      | 0.36  | —      | 0.36 | —      | 1.6   | —      | 1.6   | —      | 0.126 |
| F (units $^1$ )                             | —      | 4.4   | —      | 6.   | —      | 2.    | —      | 2.    | —      | 30.   |
| O/H (10 $^4$ )                              | —      | 6.6   | —      | 6.6  | —      | 6.6   | —      | 6.6   | —      | 6.6   |
| N/H (10 $^4$ )                              | —      | 0.5   | —      | 0.5  | —      | 0.5   | —      | 0.5   | —      | 1.    |
| Ne/H(10 $^4$ )                              | —      | 1.0   | —      | 0.8  | —      | 0.8   | —      | 0.8   | —      | 0.8   |
| S/H (10 $^4$ )                              | —      | 0.1   | —      | 0.1  | —      | 0.1   | —      | 0.1   | —      | 0.8   |
| H $\beta$ (erg)                             | —      | 0.09  | —      | 0.14 | —      | 0.036 | —      | 0.027 | —      | 0.12  |

$^1$  in  $10^{10}$  phot cm $^{-2}$ s $^{-1}$ eV $^{-1}$  at the Lyman limit ( $\alpha_{UV} = -1.5$ ,  $\alpha_X = -0.7$ );
